# Supplementary material for: Towards Interpretable Sequence Continuation: Analyzing Shared Circuits in Large Language Models
Source: arXiv:2311.04131 source file (2024-10-04)
Supplement: Supplementary file 1 [file appendix_arxivOnly.tex]

\appendix



%%%%%%%%%%%%%%%%%%%

% \textbf{Iterative Node Pruning.} We found that pruning nodes via forwards-backwards sweeps, backwards-forwards sweeps, and random sweeps (randomly removing any head) at various performance levels (node thresholds) all yielded slightly different circuits, albeit with the same important components. Thus, we only show results for the backwards-forwards sweeps.

% The circuit that is obtained from iterative ablation, and its performance score, depends on the choice of the incorrect token used in the metric and on the corrupted dataset used for ablation. 

%%%%%%%%%%%%%%%%%%%%

% \begin{figure*}[ht]
%   \centering
%   \includegraphics[scale=0.22]{diagrams/digits_numwords_circ_n80_e3_v2.pdf}
%   \caption{ A \textcolor{red}{Digits Sequence Circuit (red)}, a \textcolor{blue}{Number Words Sequence Circuit (blue)}, and \textcolor{violet}{their overlapping sub-circuit (purple, larger edges)}. The \textcolor{gray}{most important sub-circuit heads are in gray with a \textbf{bold outline}}. The digit and number words circuits achieve $\sim$70\% and $\sim$80\% performance, respectively, and the top 3\% edges are shown. 
%   }
%   \label{fig:digits_numwords_circ_n80_e3_v2}
% \end{figure*}
% % \hl{For confr vers: compare connectivities of shared nodes vs unshared}

% \begin{figure*}[ht]
%   \centering
%   \includegraphics[scale=0.25]{diagrams/bf_80n_months_digits_top3et.pdf}
%   \caption{ A \textcolor{red}{Digits Sequence Circuit (red)}, a \textcolor{blue}{Months Sequence Circuit (blue)}, and \textcolor{violet}{their overlapping sub-circuit (purple, larger edges)}. The \textcolor{gray}{most important sub-circuit heads are in gray with a \textbf{bold outline}}. The digit and months circuits achieve $\sim$70\% and $\sim$76\% performance, respectively, and the top 3\% edges are shown. }
%   \label{fig:bf_80n_months_digits_top3et}
% \end{figure*}

%%%%%%%%%%%%%%%%%%%%



%%%%%%%%%%%%%%%%%%%%

% \begin{figure*}[ht]
%   \centering
%  \includegraphics[scale=0.2]{plots/ap_late_names.png}
%   \caption{Attention Patterns for (a) Head 7.11 and (b) Head 9.1 for "among names" prompts. While at the last token (last row), head 7.11 spreads its attention out to all numbers except 1, with stronger attention to more recent numbers, head 9.1 pays strong attention to only the most recent number. }
%   \label{fig:ap_late_names}
% \end{figure*}

%%%%%%%%%%%%%%%%%%%%

% \section{Appendix A: MLP Analysis}
% \label{appendix:MLP}

% In Figure \ref{mlp_actvpath}, we utilize activation patching to find that MLP layers 9 to 11 are important. Our hypothesis is that while head 9.1 appears to play a role in determining the next sequence member, the MLP layers, namely MLP 9, also play a large role in this sub-task of sequence continuation. We also apply activation patching on individual neurons to find important neurons, as displayed in Figure \ref{mlp_actvpath_neuron}. Using prompts for increasing digit sequences, we look at neurons MLP 9 and MLP 10 to find two that stand out as “number neurons” (their contribution to the logits is only partial, so combinations of neurons are likely involved):
% \begin{itemize}
% \item Layer 9: 934 
% \item Layer 10: 1721 
% \end{itemize}

% \begin{figure*}[H]
% % \begin{figure*}[ht]
%   \centering
%   \includegraphics[scale=0.33]{plots/mlp_ap.png}
%   \caption{Activation Patching by MLP layer. MLP 9 appears to be the most important.
% }
% \label{mlp_actvpath}
% \end{figure*}

% \begin{figure*}[H]
% % \begin{figure*}[ht]
%   \centering
%   \includegraphics[scale=0.5]{plots/fig_7.pdf}
%   \caption{Activation Patching by Neuron for L10. Neuron 1721 stand out as having more than 0.2 patch improvement.
% }
% \label{mlp_actvpath_neuron}
% \end{figure*}

% Neuroscope, a tool which shows the maximum activating dataset examples for each neuron in several language models\footnote{Neuroscope was  created by Neel Nanda and can be used at: https://neuroscope.io/}, supports these findings by showing strong activations for neuron 1721 of MLP 10 near number-type tokens of several dataset examples, one of which is given in Figure \ref{fig:neuroscope}.

% \begin{figure*}[H]
% % \begin{figure*}[ht]
%   \centering
%   \includegraphics[scale=0.4]{diagrams/neuroscope.png}
%   \caption{A max activating example from the dataset for L10, N1721
% }
% \label{fig:neuroscope}
% \end{figure*}

% In future work, we will further investigate the role of MLPs for the sequence continuation tasks, such as by utilizing path patching to understand the interactions between attention heads on downstream MLPs.

\section{Dataset Details}
\label{appendix:dataset}

\textbf{Dataset Generation Procedure. } To generate each sample, we place each sequence within a specific template that is generated from an abstract template. For instance, the abstract template of '<name 1> born in <seq mem A>. <name 2> born in <seq mem B>. <name 3> born in'
% April.  was born in May.  was born in
% Russell, Grant, 
can fill in names with (Kyle, Anthony, Madison) to make a specific template. Then, the specific template can be filled in with sequence members (February, March) to create the sample 'Kyle was born in February. Anthony was born in March. Madison was born in'. We generate 1024 samples from each of three abstract templates, where each sequence (eg. 1 2 3, or 8 9 10) is represented the same number of times, for a total of 1536 samples per task. We use single tokens for all tokens in each sample. We ensure that for every sample, the model outputs the correct answer with at least twice as high probability as the incorrect answer's probability. Each specific template must also meet these required conditions for all sequences ((eg. must work for 1 2 3, 8 9 10, and two three four); else, it is not used. Each template is represented in equal proportion.

% The only exception to this condition is for "sold" template prompts for number words, in which the highest token probability is typically only 1.4 times as big as the incorrect answer's probability.

% We ensure that for every sample, the model selects the correct answer with >60\% probability, and ranks the second highest token with <20\% probability. 

% "Claire was born in February. John was born in March. Eve was born in April. Bob was born in”
We use the same templates for all tasks. For example: given the sample for the months task "Ham was bought in February. Egg was bought in March. Bread was bought in April. Steak was bought in”, we use the same non-sequence tokens to make a sample for the digits task: "Ham was bought in 2. Egg was bought in 3. Bread was bought in 4. Steak was bought in”.

The three templates we used are: <name> born in, <item> lost in, <item> done in. We choose from a set of 136 names and 100 items.

Originally, we use the token "was" in our samples (eg. "Steak was sold in March.") However, we find that the prediction outcomes were largely the same whether we included "was" or not. Thus, although "was" would make the sentences sound more natural to a human, we choose to omit it. Additionally, this allows to reduce the memory usage while running in Colab.

% For display purposes, we show these prompts with periods and the tokens "was" and "in". However, we found that the prediction outcomes were largely the same whether three tokens were used or not. Thus, to reduce the sequence length and thus memory usage while running in Colab, we omit these tokens in our datasets.

% <name> likes

% <name> has

% <item> in

% held

% Originally, we used samples such as "Austin was born in January", or "House was sold in March". However, we opt for samples using fewer tokens. We also opt for templates that made more sense in all three tasks.

% (Actually use "sold in" as the others don't elicit as high prediction on the correct token as other templates.)

% In addition to ensuring the samples were selected so that the model would output their correct answer, we also ensured the probabilities of the correct answer and second ranked token were selected with certain conditions. 
% Each task typically had different probability distributions for these templates, so we adjusted the conditions for each one. For digits, this required the correct token have >90\% probability, and have next highest token with <15\% probability. For months, this required the correct token have >70\% probability, and have next highest token with <20\% probability. For number words, this required the correct token have >60\% probability, and have next highest token with <20\% probability.

\textbf{Random Words vs Meaningful Sentences. } We find that using random words as non-sequence tokens could also allow the model to sometimes predict the next sequence member correctly. However, this did not always occur; thus, we choose to use semantically meaningful templates instead.

 % We do not permute the random words
\textbf{Sequence Member Input Positions. } We did not construct samples such that there are different intervals between the sequence members, placing them at different positions in the input (eg. "1 2 house fork 3" or "1 house fork 2 3"), because we want the model to be able to predict the next sequence member with high probability. Thus, we give it an in-context pattern where after every random word, it should predict a sequence member.

% \hl{use templates}
% \textbf{Random words vs Meaningful sentences. } We use random words rather than semantically meaningful sentences so that focus is not on any semantic parts of the input except on the sequence itself. Additionally, while there are many sentences that could use digits (eg. "1 second passed. Then, 2. 3 seconds. Finally"), we would not be able to substitute months in the same context (Eg. "January second passed" doesn't make sense). This would make our digits and months datasets less comparable. 

% Sentences in natural language would alter how sequences are continued, as additional context-dependent words such as "seconds" would have a great impact, just like how "war" and "years" had a greater impact on the greater-than task \citep{hanna2023does}. Another study may analyze these sequence continuation tasks; however, our main focus is on comparing simple sequences to find shared circuits, so we found these more elaborate tasks to be beyond the scope of this work.

% Additionally, we found that using the same word as a non-sequence member (eg. 

%%%%%%%%%%%%%%%%%%%%%%%%%%%%%
\textbf{Sequence Length. } We find that using sequences with four members allows the model to consistently obtain high probability predictions for the correct answer for all three tasks. For continuing sequences without non-sequence members, four members is usually enough to obtain a correct token probability of around 90\% or more for the three tasks, within a certain range (eg. not above twenty for number words for GPT-2). 
% Using more members typically results in a higher correct token probability.

% The samples consist of overlapping portions, such as ``1 2 3 4" and ``2 3 4 5”. These data samples are run through the model, and their activations are stored in a cache to be later analyzed via techniques such as path patching.

% we construct samplses in a similar way using a range from one to twenty, 
\textbf{Model Sequence Continuation Abilities. } For number words, as GPT-2 Small does not seem to be able to continue number word sequences higher than twenty, even when giving it the starting prefix with and without hyphens (eg. twenty or twenty- for twenty-one). We add a space in front of each number word as without the space in front, the model tokenizer would break some words greater than ten into more than one token (eg. eleven into two tokens, and seventeen into three tokens), while we aim for all our samples in a dataset to have the same number of tokens. Similarly, for digit sequences there were cases where it would break the answer into multiple tokens; for instance, in the 500-600 digit range, sometimes the next token predicted would be "5", and sometimes it would be "524". 

% \textbf{Digits Tokenization. } 
% For these cases, one may modify the input to be like "1000 1001 1002 100" so that "3" would be predicted.
% For months, we construct the dataset for January to December in a similar way to the other datasets. 

\textbf{Corrupted Dataset Details. }  We ensure that our randomly chosen sequence does not contain any elements in sequence for the last two elements of the input, as if the last two elements are not sequential, sequence continuation cannot successfully occur.
We also test variations of several corruptions other than randomly chosen tokens of a similar sequence type, such as repeats and permutations.
% We show results for ablation using randomly chosen token sequence replacement, which replaces all information about the sequence of interest to ensure none of it is present in the corrupted dataset. 
Overall, the most important components remain the same regardless of the ablation dataset and metric choices.
% Given the size of the datasets we have to work with (as only GPT-2 Small only succeeded on a limited number of sequence continuation prompts), the choice of random samples yields different performance results, but overall, the most important components remain the same regardless of the ablation dataset and metric choices.


% Using the logit difference as the performance metric, note that there are several cases where the model achieves higher performance for a task after ablating certain components. For instance, it was observed that during pruning, removing attention heads from the last few layers often improved performance. As shown by \cite{halawi2023overthinking}, we believe this may be due to ablating "overthinking" \hl{TBC}

\textbf{Other Task Datasets. } We also look for similarities between other types of tasks, such as decreasing sequences, greater-than sequences, and alphabet sequences. However, while there were a few shared circuit overlaps between these tasks and three main tasks of this paper, there were more dissimilarities. Thus, we mainly focus on the similarities of the three tasks of this paper.

% \section{Appendix ?: Details on Activation Patching and Path Patching}
% \label{appendix:actvpatch}

% Activation patching does not differentiate whether a behavior is affected by a particular component or by subsequent components downstream from paths between the component and the model's output; when they modify a component, every component that follows is impacted. In contrast, path patching lets us precisely target our intervention to a particular path. 

% \section{Appendix B: Effect of Sequence Length on Circuits}
% \label{appendix:seqlen}

% For increasing sequences of digits, we test the probability of obtaining the correct token for various sequence lengths. Figure \ref{fig:prob_seqlen} shows that a length of four is sufficient. For each x-axis value, we took the average over 10 sequences. We also notice that some sequences length of four with the first two members not-in-sequence sometimes begets correct predictions, albeit with lower logit differences. Using length-4 sequences also begets high probability for the correct token for other tasks, and for prompts using non-sequence words in between sequence words.

% \begin{figure*}[ht]
%   \centering
%  \includegraphics[scale=0.4]{plots/prob_seqlen.png}
%   \caption{Average Probability Value vs Sequence Length for Increasing Digits}
%   \label{fig:prob_seqlen}
% \end{figure*}

% \section{Appendix ?: Distribution of Attention Head Performance Drops}
% \label{appendix:dropPlot}

% We plot the histogram of attention head performance drop percentages. Each percentage drop is calculated by ablating an attention head from the full circuit, which has 100\% performance, and calculating the drop from 100\%. Heads which causes a performance increase are grouped together as heads that cause no performance change. The number of heads in each 10\% interval bin is displayed above each bin. The majority of attention heads cause little change in performance when ablating; only eight heads cause a noticable change. This suggests that most heads appear to work together, while only a few heads are important by themselves.

% \begin{figure}[h]
% % \begin{figure*}[ht]
%   \centering
%   \includegraphics[scale=0.45]{plots/hist_dropscores.pdf}
%   \caption{Histogram of attention head performance drop percentages. The number of heads in each 10\% interval bin is displayed above each bin.
% }
% \label{hist_dropscores}
% \end{figure}

%%%%%%%%%%%%%%%%%%%%%%%%%%%%%%%%%%%%%
% \section{Appendix C: Increasing Sequence Circuits Comparisons at Various Performance Levels}
% \label{appendix:perflvls}

% % \begin{figure*}[ht]
% %   \centering
% %   \includegraphics[scale=0.2]{diagrams/digits_circ_manu71n_0001e.pdf}
% %   \caption{Digits Sequence Circuit for 71\% performance. The sub-circuit nodes of Greater-Than are in yellow.
% %   }
% %   \label{fig:digits_circ_manu71n_0001e}
% % \end{figure*}

% % We do not define edges in terms of the key outputs that are used as inputs to queries; instead, the edges are shown here for demonstration purposes mainly to denote which nodes have the most effects on other nodes, as we assume all the nodes can affect one another via attention. A more detailed analysis may be performed in future work for key and query interactions for all nodes in a circuit.

% % \hl{ perf (x-ax) vs num heads/size (y-ax) ; Plot how impt heads change over perf change (which heads are dropped).  }

% In Figures \ref{fig:digits_80n_top5_perc}, \ref{fig:bf_80n_top10_nw_months}, and \ref{fig:bf_80n_top15_nw_months}, and in Tables \ref{tab:circComp_80} and \ref{tab:circHeadsComp_80}, we show results for various circuits for tasks across various performance levels. We note that as we analyze circuits for decreasing performance levels, the most important heads such as 4.4 and 9.1 remain and are not dropped. 
% % \footnote{The edges in these circuits denote how important one component is for another, similar to the graphs found in \cite{conmy2023towards}. One component can affect another component by using different subspaces of the residual stream \citep{elhage2021mathematical}. This is why the edges are not required to only be between components in adjacent layers.} 

% Lastly, in Figure \ref{fig:all_tasks_intersect_80n_3e}, we display the sub-circuit defined as the intersection of the three circuits from Figure \ref{fig:all_tasks_80n_3e_overlapE}. We note that this sub-circuit alone, despite being important, is not enough to achieve high performance (> 60\%) in any of these tasks, indicating that the other "less essential" components, when put together, are still very important.

% \begin{figure*}[ht]
%   \centering
%   \includegraphics[scale=0.12]{diagrams/digits_80n_top5_perc.pdf}
%   \caption{ An Increasing Digits Sequence Circuit that achieves $\sim$80\% performance, with the top 5\% edges are shown. The \textcolor{violet}{most important sub-circuit heads are in purple.} Note that at an edge threshold of 5\%, there are still three nodes without any edges; however, we still include them in the figure to show all the nodes found via iterative ablation for a digits circuit using a node threshold of 80\%.
%   }
%   \label{fig:digits_80n_top5_perc}
% \end{figure*}

% \begin{figure*}[ht]
%   \centering
%   \includegraphics[scale=0.25]{diagrams/bf_80n_top10_nw_months.pdf}
%   \caption{ A \textcolor{red}{Number Words Sequence Circuit (red)}, a \textcolor{blue}{Months Sequence Circuit (blue)}, and \textcolor{violet}{their overlapping sub-circuit (purple, larger edges)}. The \textcolor{gray}{most important sub-circuit heads are in gray with a \textbf{bold outline}}. The number words and months circuits achieve $\sim$80\% and  $\sim$76\% performance, respectively, and the top 10\% edges are shown.
%   }
%   \label{fig:bf_80n_top10_nw_months}
% \end{figure*}

% \begin{figure*}[ht]
%   \centering
%   \includegraphics[scale=0.24]{diagrams/bf_80n_top15_nw_months.pdf}
%   \caption{ A \textcolor{red}{Number Words Sequence Circuit (red)}, a \textcolor{blue}{Months Sequence Circuit (blue)}, and \textcolor{violet}{their overlapping sub-circuit (purple, larger edges)}. The \textcolor{gray}{most important sub-circuit heads are in gray with a \textbf{bold outline}}. The number words and months circuits both achieve $\sim$80\% performance, respectively, and the top 15\% edges are shown. Note the contrast of the graph size to the circuit in Figure \ref{fig:bf_80n_top10_nw_months}, which only keeps the top 10\% of edges. We keep the head without edges, 8.9, in the figure.
%   }
%   \label{fig:bf_80n_top15_nw_months}
% \end{figure*}

% % \toprule
% % Important Head &  Digits & NumWords & Months & Greater-Than \\
% % \midrule
% % 4.4 & -35.95\% & -22.48\% & -51.35\% & 10\% \\
% % 9.1 & -20.44\% & -27.15\% & -53.32\% & 10\% \\
% % 7.11 & -12.13\% & -14.59\% & -30.37\% & 10\% \\
% % % 7.10 & -2.75\% & -2.66\% & N/A & 10\% \\
% % % 8.11 & -10.24\% & -6.08\% & -8.84\% & 10\% \\
% % 1.5 & -16.32\% & - & - & - \\
% % % 10.2 & - & -12.40\% & - & - \\
% % \bottomrule

% \renewcommand{\arraystretch}{1.5}
% \begin{table*}[ht]
% \centering
% \caption{Performance scores for tasks (cols) run on similar tasks' $\sim$80\% circuits (rows)}
% \vspace{0.5em} % Adds vertical space between caption and table
% \begin{tabular}{c|cc cc|c}
% \toprule
%   & Digits Task & NumWords Task & Months Task \\
% \hline
% Digits Circuit & 80.20\% &  55.55\% & 69.71\% \\
% Words Circuit & 35.10\% &  80.20\% & 70.61\% \\
% Months Circuit & 16.23\% &  50.24\% & 80.02\% \\
% \hline 
% % Random & $\mu=0.9, \sigma=0.4$ & $\mu=1, \sigma=0.4$ & $\mu=1.4, \sigma=0.8$ & $\mu= -0.85, \sigma=0.43$ \\
% \toprule
% \end{tabular}
% \label{tab:circComp_80}
% \end{table*}

% % Digits Circuit & 82.95\% &  74.75\% & TBD & 64.12\% & TBD \\
% % Words Circuit & 48.09\% &  81.98\% & TBD & 81.77\% & TBD \\
% % Months Circuit & 28.45\% &  36.09\% & TBD & 48.05\% & TBD \\
% % GreaterThan Circuit & 12.54\% &  20.85\% & TBD & 85.38\% & TBD \\
% % % DecrDig & TBD & TBD & TBD & TBD & TBD & TBD \\
% % % \midrule 
% % \hline 
% % % \bottomrule 
% % IOI Circuit & 2.08\% &  12.27\% & TBD & 28.52\% & TBD \\

% % IOI (w/ ABC as mean)

% \begin{table*}[ht]
%     \centering
%     \caption{Drop in Performance for each Task When the Important Head is Removed from Circuit with 80\% Performance using Random Token Ablation. This is not a drop from 100\%, but from $\sim$80\% (e.g. -56\% means a drop from 80\% to 24\%) }
%     \vspace{0.5em} % Adds vertical space
%     \begin{tabular}{c|ccccc}
%         \toprule
%         Important Head &  Digits & NumWords & Months \\
%         \midrule
%         4.4 & -56.00\% & -32.15\% & -59.18\% \\
%         9.1 & -46.75\% & -45.72\% & -58.98\% \\
%         7.11 & -24.61\% & -20.39\% & -14.56\% \\
%         % 7.10 & -2.75\% & -2.66\% & N/A & 10\% \\
%         % 8.11 & -10.24\% & -6.08\% & -8.84\% & 10\% \\
%         1.5 & -25.45\% & -12.28\% & - \\
%         % 10.2 & - & -12.40\% & - & - \\
%         \bottomrule
%     \end{tabular}
% \label{tab:circHeadsComp_80}
% \end{table*}
% % This is not a percentage from 80\%, but from the full score (using the entire unablated model) 

% \begin{figure*}[ht]
%   \centering
%   \includegraphics[scale=0.5]{diagrams/all_tasks_intersect_80n_3e.pdf}
%   \caption{ The sub-circuit defined as the intersection of the three circuits from Figure \ref{fig:all_tasks_80n_3e_overlapE}. The Digits, Number Words, and Months circuits achieve $\sim$70\%, $\sim$80\%, and $\sim$76\% performance, respectively, and the top 3\% edges are shown.
%   }
%   \label{fig:all_tasks_intersect_80n_3e}
% \end{figure*}

%%%%%%%%%%%%%%%%%%%%%%%%%%%%%%%%%%%%%

% \begin{figure*}[ht]
%   \centering
%   \includegraphics[scale=0.225]{diagrams/all_tasks_80n_3e_overlapE.pdf}
%   \caption{ A \textcolor{red}{Digits Sequence Circuit (red)}, a \textcolor{blue}{Number Words Sequence Circuit (blue)}, a \textcolor{gold}{Months Sequence Circuit (gold)}. The overlapping sub-circuit parts are coded as follows: \textcolor{violet}{Digits and Number Words only are in purple}, \textcolor{orange}{Digits and Months only are in orange}, \textcolor{darkgreen}{Number Words and Months only are in green}, and \textcolor{lightgray}{All Three Tasks are in white} with \textbf{black edges}. The \textcolor{gray}{most important sub-circuit heads are in gray with a \textbf{bold outline}}. The Digits, Number Words, and Months circuits achieve $\sim$70\%, $\sim$80\%, and $\sim$76\% performance, respectively, and the top 3\% edges are shown. }
%   \label{fig:all_tasks_80n_3e_overlapE}
% \end{figure*}

% Lastly, in Figure \ref{fig:all_tasks_intersect_80n_3e}, we display the sub-circuit defined as the intersection of the three circuits from Figure \ref{fig:all_tasks_80n_3e_overlapE}. We note that this sub-circuit alone, despite being important, is not enough to achieve high performance (> 60\%) in any of these tasks, indicating that the other "less essential" components, when put together, are still very important.
% test its performance on each task?

% \section{Appendix ?: Ablation via Repeated Sequence Corruption}
% \label{appendix:repeated}

% \FloatBarrier

% \section{Appendix D: Comparisons to Greater-Than Circuits}
% \label{appendix:greater}

% We reproduce the results of \cite{hanna2023does} using our approach. Figure \ref{fig:gt_circuits}(a) shows the results of path patching on the heads from \cite{hanna2023does} using a 10\% edge threshold.. We found that this circuit achieves 85\% performance using our ablation and performance metric approach. In Figure \ref{fig:gt_circuits}(b), we also obtain an alternative circuit which achieves 97\% accuracy for greater-than using our iterative ablation method. it has considerable overlap with the circuit in Figure \ref{fig:gt_circuits}(a). Lastly, in Figure \ref{fig:digit_gt_top3_15_97n}, a Digits Circuit for $\sim$70\% performance with a 3\% edge threshold and a Greater-Than Circuit for $\sim$97\% performance with a 15\% edge threshold are shown together, demonstrating some overlapping components such as heads 0.5, 5.1, 6.9, and 9.1.

% % \begin{figure*}[ht]
% %   \centering
% %   \includegraphics[scale=0.4]{diagrams/gt_orig_top10_perc.pdf}
% %   \caption{A Greater-Than Circuit for $\sim$85\% performance, using the heads found by \cite{hanna2023does} and a 10\% edge threshold
% %   }
% %   \label{fig:gt_orig_top10_perc}
% % \end{figure*}

% % \begin{figure*}[ht]
% %   \centering
% %   \includegraphics[scale=0.4]{diagrams/gt_bf97_top15_perc.pdf}
% %   \caption{A Greater-Than Circuit for $\sim$97\% performance, found via iterative pruning and a 15\% edge threshold
% %   }
% %   \label{fig:gt_bf97_top15_perc}
% % \end{figure*}

% \begin{figure*}[ht]
%   \centering
%   \includegraphics[scale=0.3]{diagrams/gt_circuits.png}
%   \caption{ (a) A Greater-Than Circuit for $\sim$85\% performance, using the heads found by \cite{hanna2023does} and a 10\% edge threshold, (b) A Greater-Than Circuit for $\sim$97\% performance, found via iterative pruning and a 15\% edge threshold
%   }
%   \label{fig:gt_circuits}
% \end{figure*}

% \begin{figure*}[ht]
%   \centering
%   \includegraphics[scale=0.2]{diagrams/digit_gt_top3_15_97n.pdf}
%   \caption{ \textcolor{red}{A Digits Circuit (red)} for $\sim$70\% performance with a 3\% edge threshold and \textcolor{blue}{a Greater-Than Circuit (blue)} for $\sim$97\% performance with a 15\% edge threshold. The most important node shared by the two circuits is head 9.1.
%   }
%   \label{fig:digit_gt_top3_15_97n}
% \end{figure*}

% % \FloatBarrier

% \section{Appendix E: Comparisons to Decreasing Digits Circuits}
% \label{appendix:decr}

% % \hl{move a paragraph of this, possibly diagram, to main paper and move other details to appendix}

% We use decreasing digit sequences of length 8 in order to achieve a >90\% probability output for the correct token for most prompts, as for increasing digit sequences, we use sequences of length 4 to achieve a >90\% probability output for the correct token for most prompts.

% As shown in Figure \ref{fig:decr_incr_80n}, the decreasing digits circuit is first found via iterative node pruning using an 80\% threshold. Then, its edges are found via path patching using a 3\% edge threshold. Afterwards, 7 heads are dropped, decreasing the performance to $\sim$60\%. We display this circuit with decreased performance instead of the one at 80\% with a higher edge threshold for readability purposes.

% This circuit does not share nodes that are crucial for increasing sequence continuation, such as head 9.1. This fits with our observation that 9.1 has high "next" scores. Thus, we use OV unembedding to look for heads with high "previous" output component scores in which the input of a digit causes the previous digit to be predicted; however, though there were several heads with decently high "previous member" output component scores (around 50-60\%), we did not find heads such as 9.1 with very high previous member scores that were higher than their copy and next member scores (head 9.1 had a next member score $\sim$87\%, which was much higher than its copy score). Therefore, we did not locate "previous member" heads. We hypothesize that role of determining the next token in a decreasing token may be more distributed across several components, rather being more concentrated to some "previous member" head.

% Table \ref{tab:decrHeadsComp} shows that there are many heads that are very important for the decreasing circuit performance; even just dropping head 4.10 destroys the entire performance! We also note that only head 7.11 is considered an important head in both the decreasing and increasing digits circuits. Further investigation of why this occurs will be done in the future.

% \begin{figure*}[ht]
%   \centering
%   \includegraphics[scale=0.2]{diagrams/decr_incr_80n.pdf}
%   \caption{ \textcolor{red}{An Increasing Digits Circuit (red)} for $\sim$70\% performance with a 3\% edge threshold and \textcolor{blue}{a Decreasing Digits Circuit (blue)} for $\sim$60\% performance with a 3\% edge threshold. The heads 1.5, 7.11, and 9.1 are in gray; however, only head 7.11 is important for both the decreasing and increasing digits circuits.
%   }
%   \label{fig:decr_incr_80n}
% \end{figure*}

% \begin{table*}[ht]
%     \centering
%     \caption{Drop in Performance for each Task When the Important Head is Removed from Decreasing Digits Circuit with 80\% Performance using Random Token Ablation. This is not a drop from 100\%, but from $\sim$80\% (e.g. -56\% means a drop from 80\% to 24\%) }
%     \vspace{0.5em} % Adds vertical space
%     \begin{tabular}{c|ccccc}
%         \toprule
%         Important Head & Decr Digits  \\
%         \midrule
%         4.10 & -87.39\% \\
%         7.11 & -64.61\% \\
%         7.10 & -38.55\% \\
%         5.1 & -38.54\% \\
%         4.11 & -31.29\% \\
%         6.10 & -26.48\% \\
%         9.5 & -25.45\% \\
%         \bottomrule
%     \end{tabular}
% \label{tab:decrHeadsComp}
% \end{table*}

% % \hl{decr digits/etc. has diff impt heads that DON'T seem to correspond to "previous member heads" }
% % Thus, we look for heads with high "previous" scores. We find that head 6.9 has high previous scores; however, 6.9 also has high next scores. This implies that head 6.9 is not exclusively a "previous" sequence continuation head, while head 9.1 does seem to specialize in "next" outputs.
% % \textbf{Previous Sequence Scores. } \hl{TBD}

% \textbf{Less-Than Circuit. } \cite{hanna2023does} reports that GPT-2 Small was unable to perform Less-Than tasks correctly. We attempt several methods, such as using in-context examples or common dataset patterns that often use less-than (similar to how Greater-Than uses the common dataset pattern of a war lasting from a start year to a end year), to try to get the model to perform well on Less-Than tasks variations, but we did not find that a Less-Than task it was able to succeed with.
% % \textbf{Less-Than Circuit. } \cite{hanna2023does} also found that the greater-than circuit was incorrectly used for less-than prompts... However, we use in-context learning to allow the model to perform less-than tasks...

% \section{Appendix ?: Alphabet Continuation Task Connectivity}

% We did not compare with the alphabet sequences as it does not share many heads with the others. 

% \section{Appendix ?: Layer-wise Functionality Analysis}

% \FloatBarrier

\section{MLP Functionality Analysis Details}
\label{appendix:MLP}

When using an analysis similar to component output scores, we do not find that MLP 9 outputs next sequence members when given member(s) of a sequence. We hypothesize that its role is more nuanced than simply acting as a key:value store for next sequence members, and requires more work to decipher \footnote{We plan to perform more neuron-level and feature-level analysis for this in future work.}.

\section{Iterative Method Details. }
\label{appendix:itermethod}

Instead of absolute impact on performance score, we can also use relative impact. This means that the removal won’t cause it to go down by more than 0.01 of the existing score, rather than an absolute threshold of 80\%. However, this still doesn’t take combos into account. one edge removal may make it 0.01, and another 0.01, but doesn’t mean their combined effect is also 0.02; it may be more. Thus, order of removal may have an impact on the circuit.

\section{Extended Results of Important Head Functionality}
\label{appendix:imptHeads}

In this section, we show other attention patterns for various task and head combinations.

% \begin{figure*}[ht]
%   \centering
%  \includegraphics[scale=0.4]{plots/attnpat1_5_among_months.pdf}
%   \caption{Attention Patterns for Head 1.5. Lighter colors mean higher attention values. It is considered a month detection head as months attend to months. The abbreviated months are shown for demonstration purposes, but the results are similar for both full month words and their abbreviations. For each of these detection patterns, query is shown in green, and the key is shown in blue. }
%   \label{fig:attnpat1_5_among_months}
% \end{figure*}

\begin{figure*}[ht]
  \centering
 \includegraphics[scale=0.2]{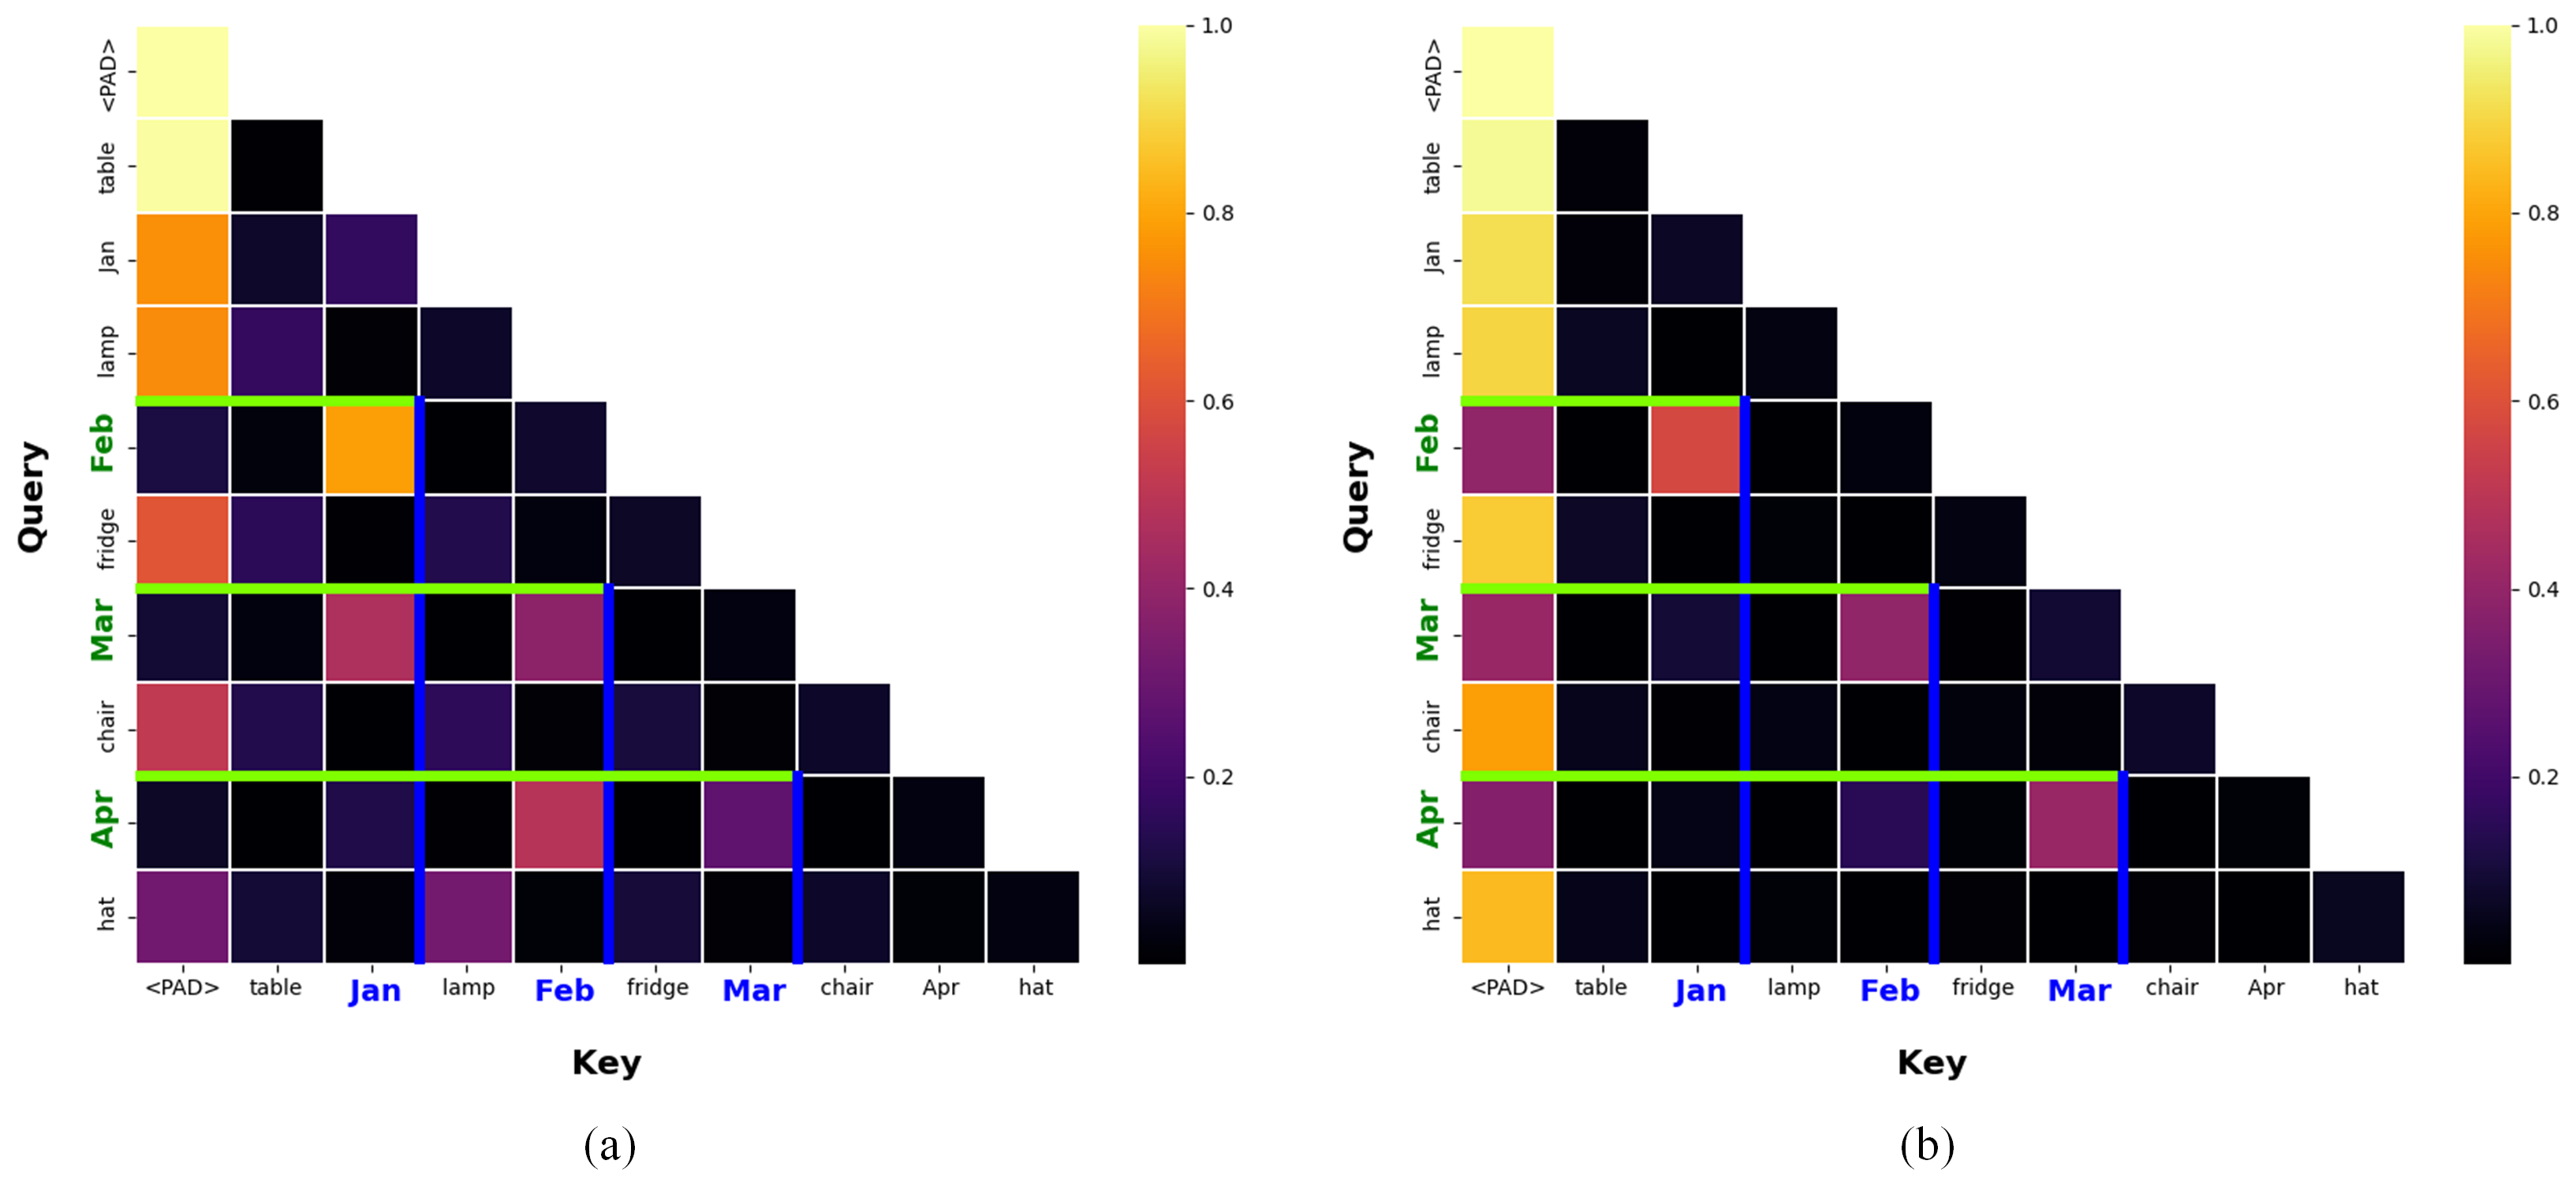}
  \caption{Attention Patterns for (a) Head 1.5 and (b) Head 4.4. They are considered month detection heads as months attend to months. The abbreviated months are shown for demonstration purposes, but the results are similar for both full month words and their abbreviations. Though the drop in performance was higher for the months circuit than for the digits circuit when head 4.4 was removed, there are other explanations aside from head 4.4 being more important for months, such as the digits circuit having backup paths. }
  \label{fig:attnpat_early_mixed_months}
\end{figure*}

\begin{figure*}[ht]
  \centering
 \includegraphics[scale=0.2]{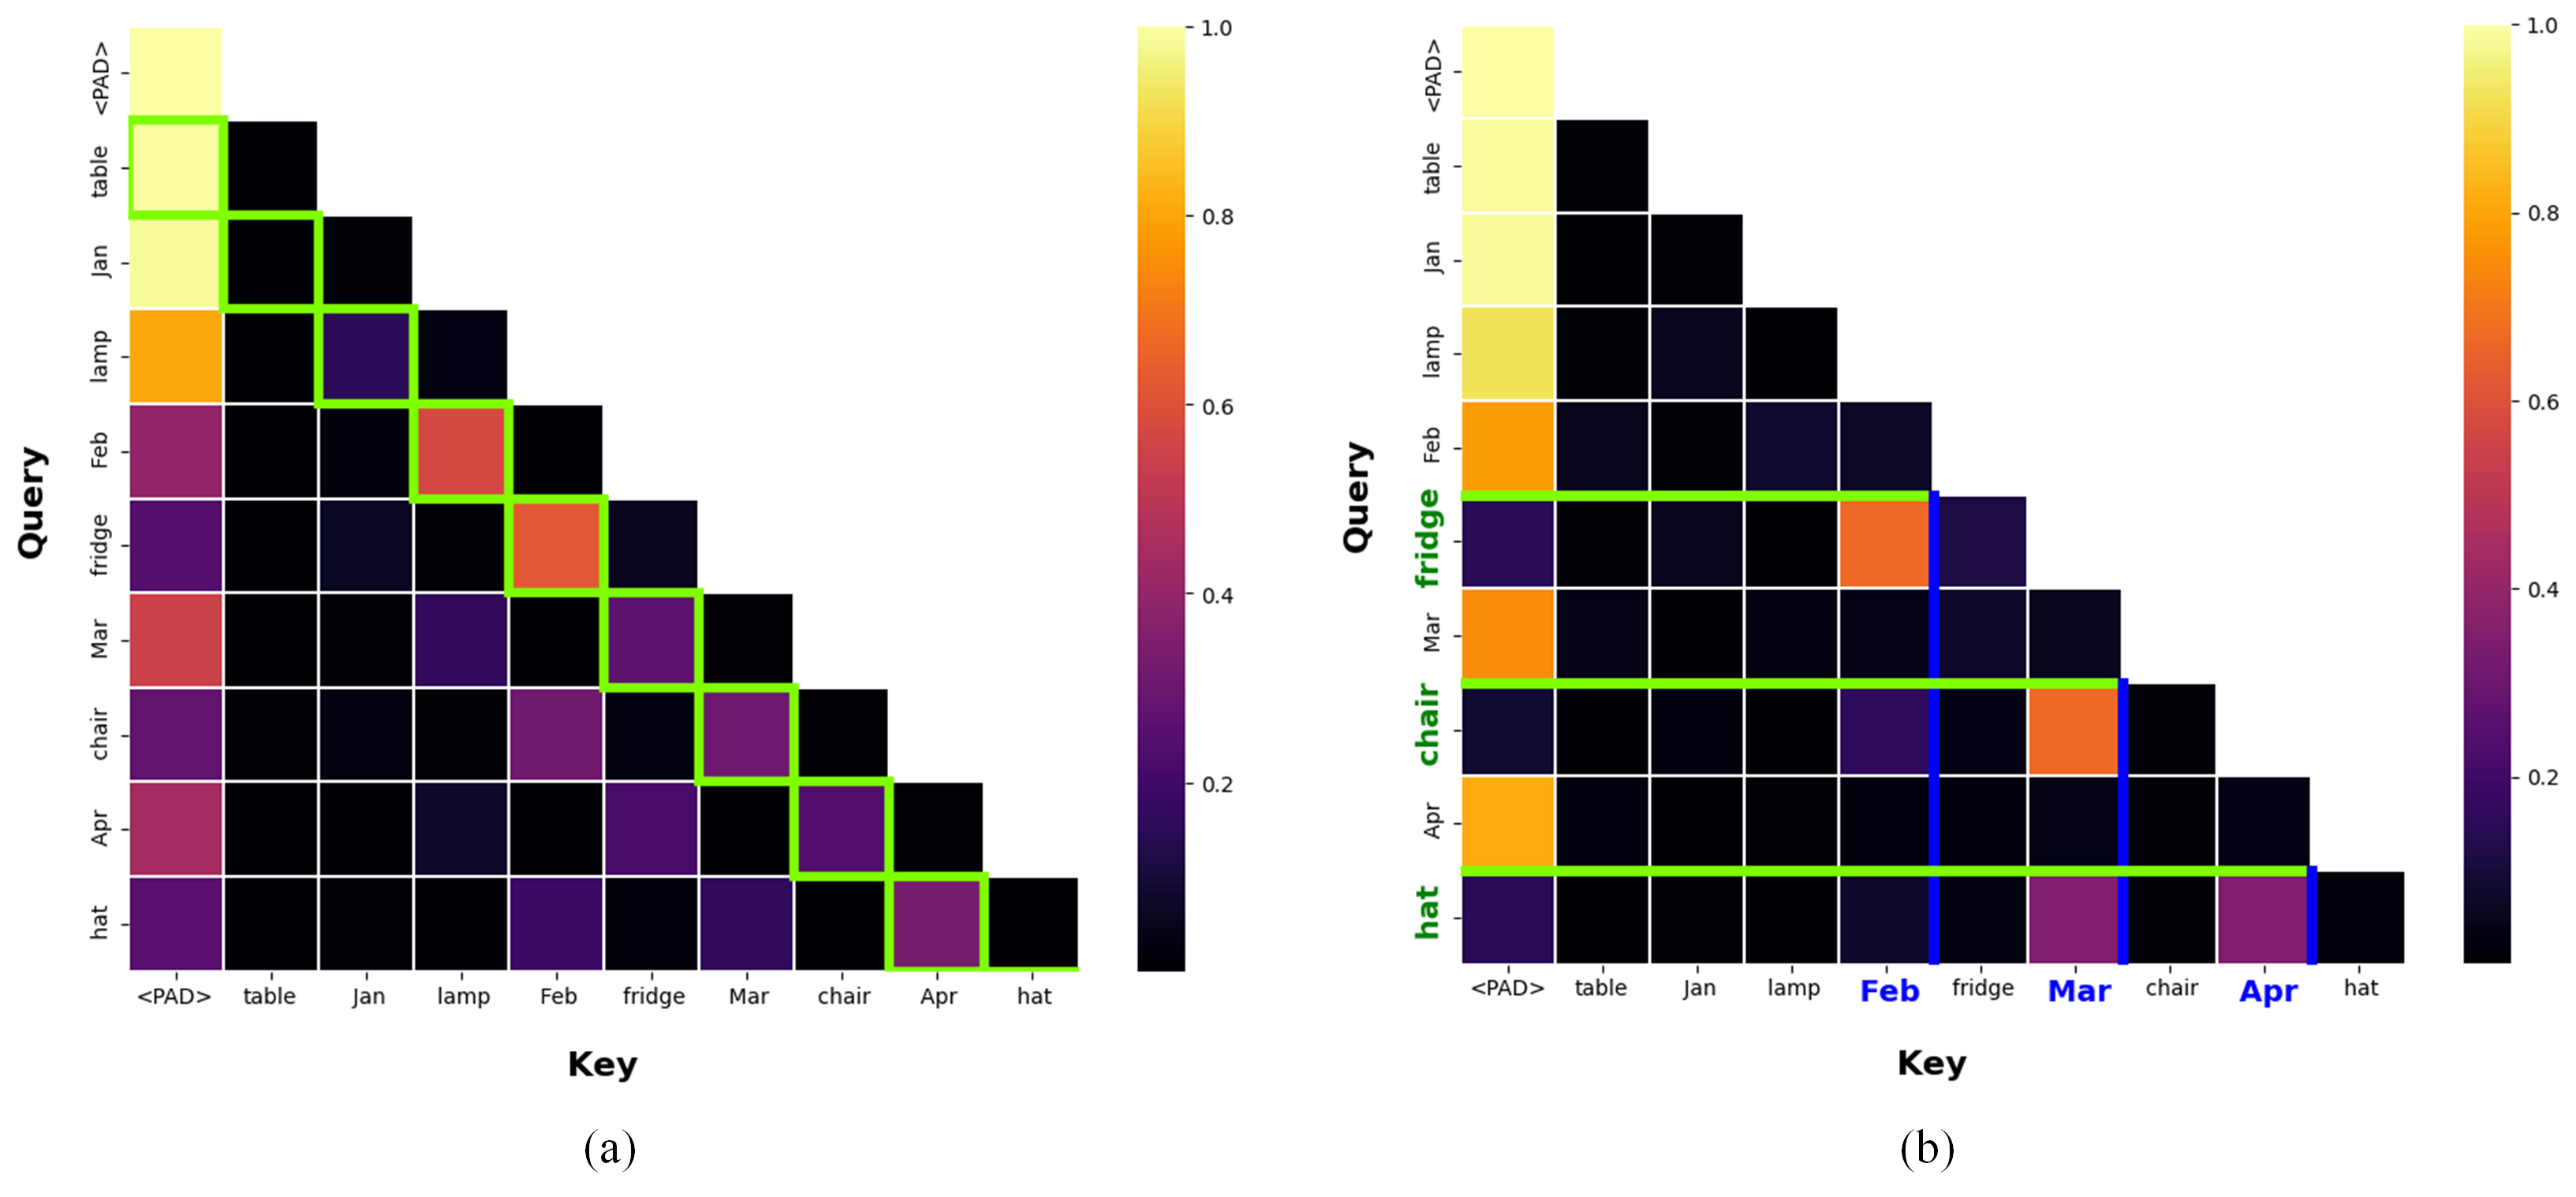}
  \caption{Attention Patterns for (a) Head 7.11 and (b) Head 9.1. Lighter colors mean higher attention values. We observe that 9.1's role for attending to the last month may not be as strong as its role for the last digit and last number word. }
  \label{fig:attnpat_late_mixed_months}
\end{figure*}

\begin{figure*}[ht]
  \centering
 \includegraphics[scale=0.2]{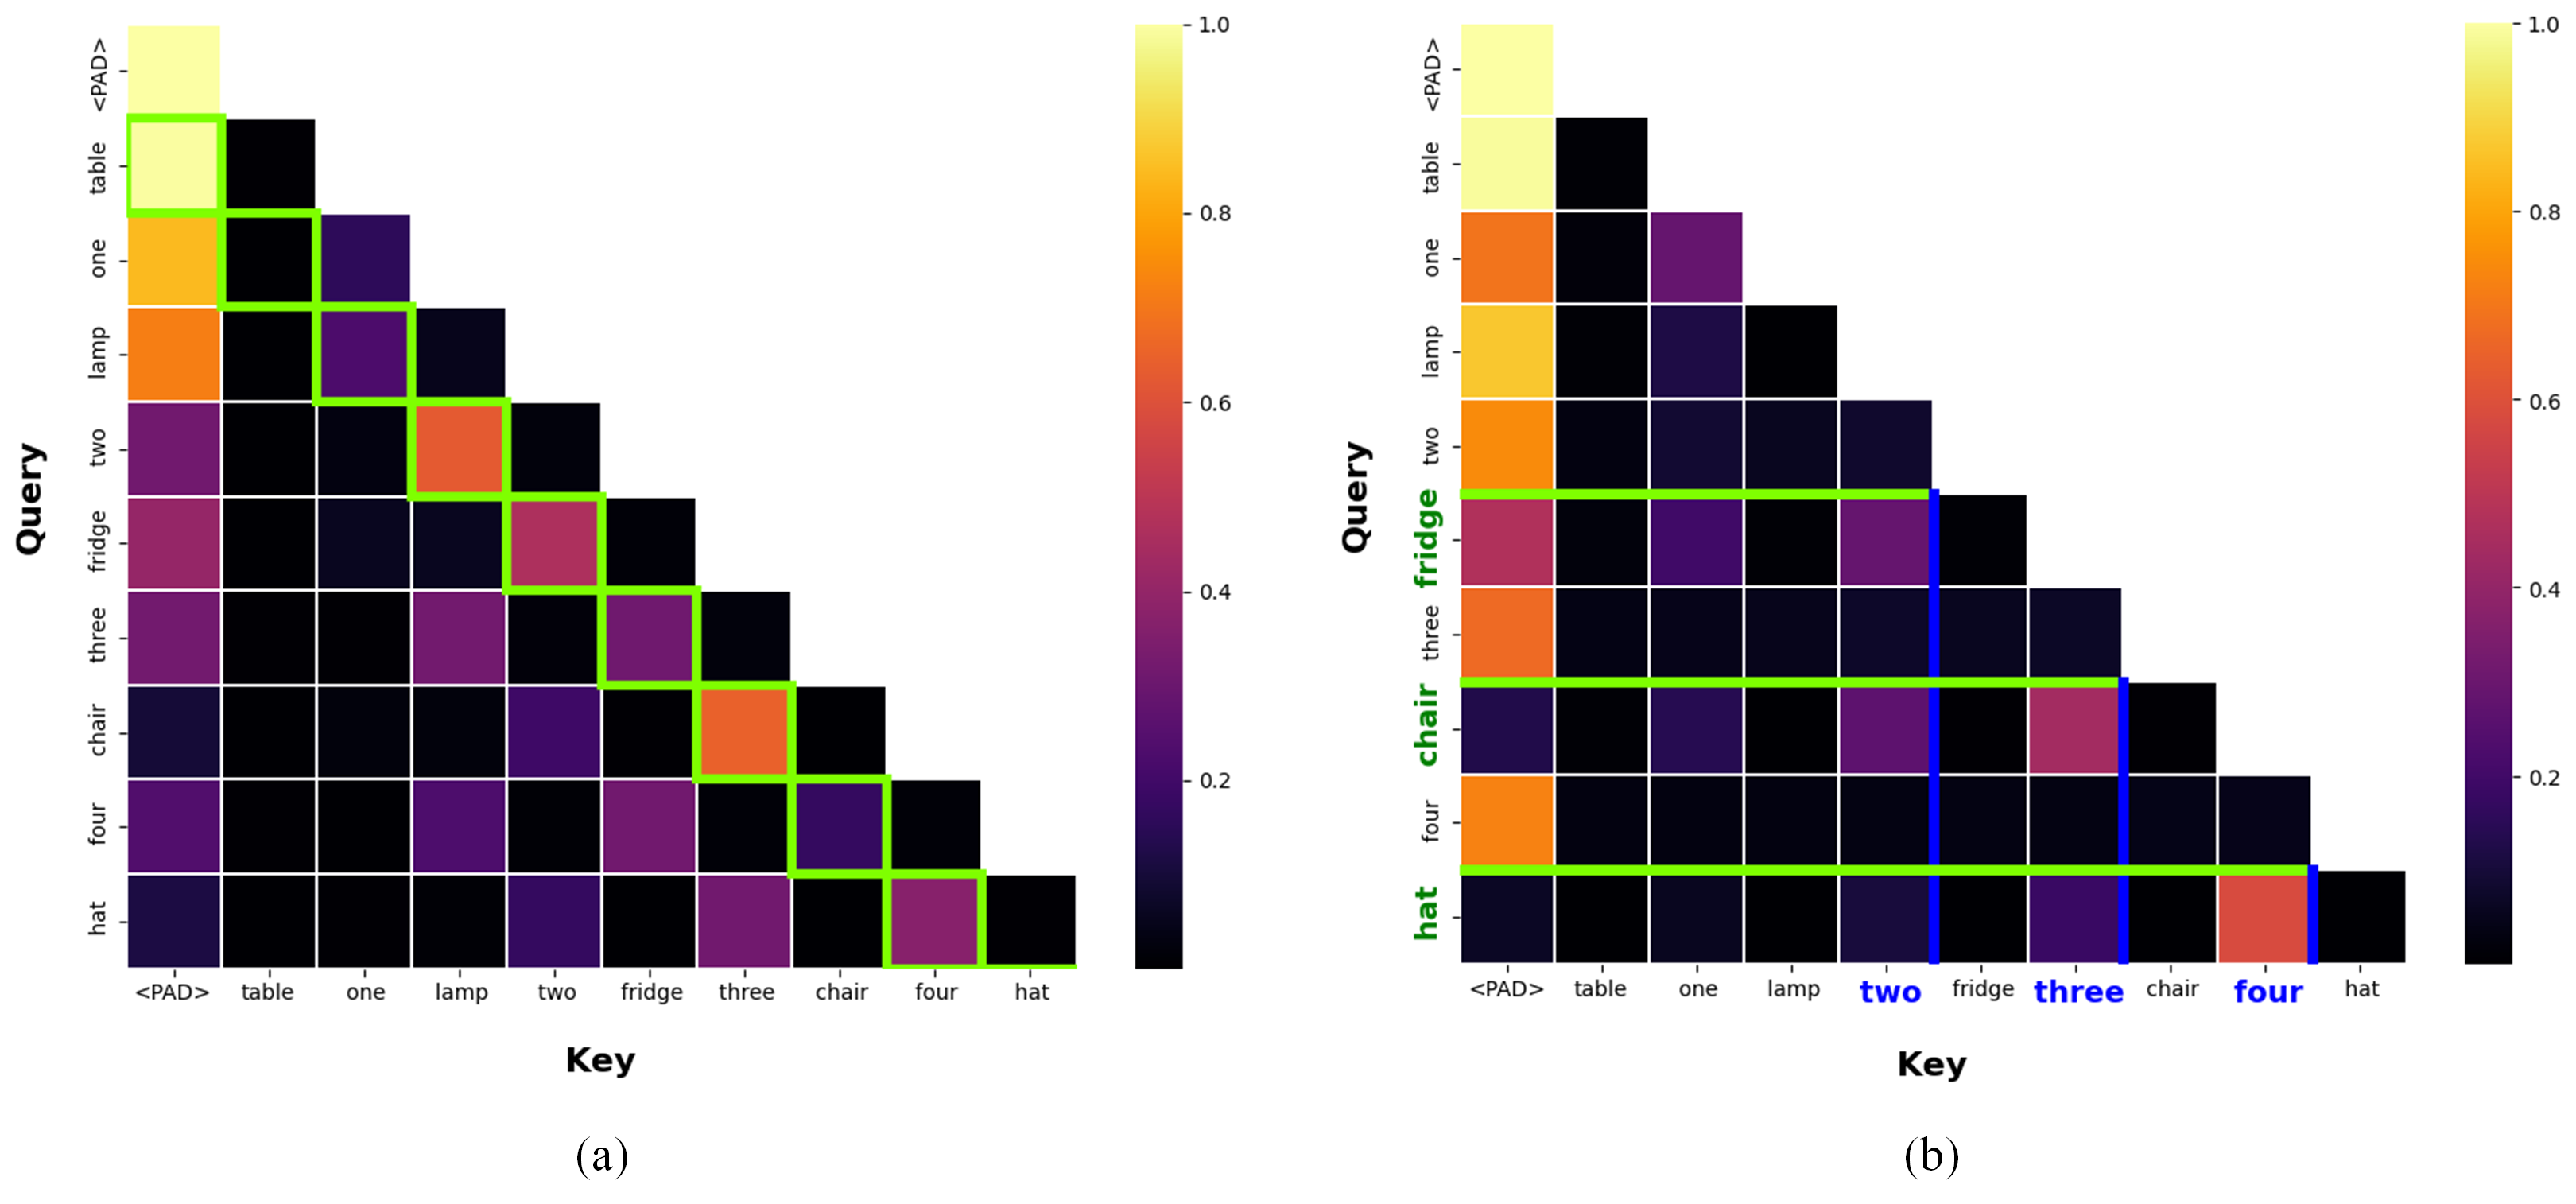}
  \caption{Attention Patterns for Number Words of (a) Head 7.11 and (b) Head 9.1. Lighter colors mean higher attention values. The abbreviated months are shown for demonstration purposes, but the results are similar for both full month words and their abbreviations. For each of these detection patterns, query is shown in green, and the key is shown in blue. }
  \label{fig:attnpat_late_mixed_nw}
\end{figure*}

% \FloatBarrier

% \section{Appendix G: Other Early Head Analysis: Similar Type, Previous Token, Induction Heads}
% \label{appendix:earlyheads}

% \cite{wang2022interpretability} discovered attention heads in early layers that functioned as the following types:
% % \emph{Duplicate Heads}, \emph{Induction Heads}, and \emph{Previous Token Heads}. 

% \begin{itemize}
%     \item \emph{Duplicate Token Heads} transfer the position of a previously occurring duplicate token to its current location.
%     % , assessing if the sequence focuses on prior instances with an offset of $n$. 
%     % determine attention patterns by evaluating sequences of random tokens of length $n$. 
%     \item \emph{Induction Heads} predict that token $[B]$ follows token $[A]$ based on previous patterns of $[A] [B]$. 
%     % In other words, given the sequence $[A][B]...[A]$, induction heads aid in predicting $[B]$ as the next token.
%     % They are determined by evaluating attention patterns with an offset of $n-1$, meaning the second occurrence of a token $[A]$ focuses on the token $[B]$ that follows its first instance. 
%     \item \emph{Previous (n-k) Token Heads} work in tandem with Induction Heads by storing information about $[A]$ in the residual stream at the position $[B]$. 
%     % This enables Induction Heads to recognize the next appearance of $[A]$ and align it with that position, subsequently transferring $[B]$ to the output.
% \end{itemize}

% % Additionally, we identify two new categories of heads called "Similar Type Heads" and "Previous (n-k) Token Heads". We run experiments where similar types are spaced out by different lengths in between them to ensure that "Similar Type Heads" are not "Previous (n-k) Token Heads". We found that some may function as both types. 
% % \cite{wang2022interpretability} notes that heads 0.1 and 0.10 are duplicate token heads in the context of IOI; our results agree with theirs.
% % ; for our case, we note they play a broader role, acting as "similar type" heads.

% % Figure \hl{TBD} obtains the duplicate token scores, previous token scores, and induction scores for every head in GPT-2 Small. It matches Figure 18 in \cite{wang2022interpretability}. We take the early layer heads hypothesized to be of these types and check their scores. The Early Layer Heads appear to be categorized as follows: \hl{may turn into table or venn diagram}

% \begin{itemize}
%     \item Duplicate: 0.1,  0.5, 0.10 (stated to be fuzzy in IOI)
%     % \item Duplicate/Similar Type: ???
%     % \item Number Sequence Detection: 1.5, 4.4
%     \item Previous Token: 0.3 (only n-1 and n-2 on period?)
%     % , 1.5 (was prev for IOI?)
%     \item Induction: 5.5, 6.1 (?), 6.9
%     % \item ??? : 0.3 (only n-1 and n-2 on period?)
%     % \item Multi-Role: 1.5???
% \end{itemize}

% \emph{Identifying Early Heads by Attention Patterns}: The attention patterns of the digits sequences are mostly the same for all its top heads; they attend stronger to more recent numbers. This is unsurprising, as our test prompts find that “corrupting” tokens before the last or second last still allows the model to complete the sequence correctly, indicating those two tokens are by far the most important, though the ones before do still contribute to the logit of the correct output. \hl{move this to appendix next to 'vary seq len' vs logit}

% \emph{Identifying Early Heads by Attention Patterns Among Words}: We notice that Early Heads attend to previous tokens of exactly the same or similar types. For instance, Figure \ref{fig:attnpat15and44} shows number detection heads 1.5 and 4.4, where digit tokens attend to digit tokens. These are considered number detection head as numbers attend to numbers, but other token types do not attend to their similar types; for instance, names do not attend to names. In contrast to the similar token heads, head 1.5 does not appear to be significant for the pure digit sequence circuit. \hl{show plot of 1 head in main, then link to side-by-side smaller plots of other heads in APpendix}

% These heads also appear to either attend to the previous (n-1) token or the (n-2) token. This suggests these heads are either ‘n-k position’ detection or 'similarity detection' heads. The pure sequence experiments with the same heads show that these heads do not always attend to (n-1) or (n-2), however; they attend to the same token type, regardless of its position. For instance, head 0.1 does not attend to the previous (n-2) token in the pure sequence case. Head 4.4 attends to the previous number in the pure sequence case, while it also attends to the previous number in the impure case, in which the previous number is not at the previous token position from the number token acting as the query.  Thus, these heads appear to be "similarity detection heads". \hl{show the pure fig; likely move this reasoning to appendix}

% The induction heads are heads 5.5, 6.1, and 6.9. This is considered an induction head as for the pattern "[name] is [number].", which has n=4 tokens, each token attends to the token (n-1)=3 positions before, which is right before its previous counterpart in the pattern. The induction head pattern can be seen in the attention pattern for head 6.1 in Figure \ref{fig:attnpat61}. Previous papers found that heads 5.5 and 6.9 were induction heads, but not head 6.1 \citep{wang2022interpretability}. \hl{6.1 may be 'weak induction'} 
% % \hl{consistent offset not as strong in 6.1 as in others; it may be 'weak induction'} 

% \begin{figure*}[ht]
%   \centering
%  \includegraphics[scale=0.3]{plots/attnpat61.pdf}
%   \caption{Attention Pattern for Head 6.1. This is considered an induction head as for the pattern "[name] is [number].", which has n=4 tokens, each token attends to the token (n-1)=3 positions before, which is right before its previous counterpart in the pattern. This offset pattern is highlighted in green.}
%   \label{fig:attnpat61}
% \end{figure*}

%%%%

% \textbf{Comparison to Greater-Than Circuit.} The greater-than early heads are heads 0.1, 0.3, and 0.5. These heads, along with MLPs 0 to 3, were stated by \citep{hanna2023does} to read in "YY", the last two the numerical digits of a four-digit year, and may be considered as "number detection heads", a type of similarity detection head. Incidentally, we find that heads 0.1 and 0.5 are also duplicate heads, and that head 0.3 appears to be a previous token head, but attends only from the period (".") token. Number sequence detection heads 1.5 and 4.4 do not appear to be important for the greater-than task, as that input types does not contain a sequnece of numbers.

% \section{Appendix ?: Attention Patterns Of Shared Heads}
% \label{appendix:attnpat}

% \section{Appendix G: Attention vs Output Value Correlation}
% \label{appendix:attnVSov}

% \textbf{Attention vs Output Value Correlation. } 
% In Figure \ref{9.1_scatter}, for digit tokens between 1 to 100, we plot the relationship of their attention vs output value for head 9.1 to check copy scores, an approach used by \cite{wang2022interpretability}. The x-axis represents the  (<end>, S) value of the QK matrix; that is, the attention that <end> pays to token S. The y-axis represents how much token S contributes to the output value of the attention head. This measures the strength of the correlation between when <end> attends to S, and how strong the output will be “composed of” S (in the case of copy scores, this means outputting S with high logits). 
% We observe there to be strong correlation, indicating that this head 9.1 is detecting numbers. Similar patterns can be seen when passing in month token inputs, as seen in Figure \ref{scatter_months_9.1}. The correlation scores of several heads is given in Table \ref{table:corrScores}.
% % in Appendix \ref{appendix:OVscores}.  

% \begin{figure*}[ht]
%   \centering
%   \includegraphics[scale=0.5]{plots/fig_3.pdf}
%   \caption{Writing Direction Scatterplot for tokens in digit sequences, head 9.1
% (Correlation: 0.8128, p-value: 8.9942e-70)
% }
% \label{9.1_scatter}
% \end{figure*}


% \begin{figure*}[H]
%   \centering
%   \includegraphics[scale=0.5]{plots/fig_6.pdf}
%   \caption{Writing Direction Scatterplot for tokens in month sequences, head 9.1
% (Correlation: 0.9307, p-value: 4.3906e-11)
% }
% \label{scatter_months_9.1}
% \end{figure*}

% \begin{table*}[h]
%     \centering
%     \renewcommand{\arraystretch}{1.25} % Adjusts the height of each row
%     \caption{Correlation Scores of Attention Heads with Ordered Sequences}
%     \vspace{0.5em} % Adds vertical space between caption and table
%     \label{table:corrScores}
%     \begin{tabular}{ccc}
%         \hline
%         \textbf{Head} & \textbf{Digits} & \textbf{Months} \\
%         \hline
%         9.9 & 0.81 & 0.93 \\
%         9.1 & 0.77 & 0.75 \\
%         7.10 & 0.89 & 0.92 \\
%         5.1 & 0.64 & 0.71 \\
%         0.3 & 0.09 & 0.13 \\
%         \hline 
%     \end{tabular}
% \end{table*}

%%%%%
% \FloatBarrier

% \textbf{Similar Token Sequence Scores. } A head may not be outputting the exact same token or an adjacent token, but it may be outputting a similar type of token; for sequence-type tokens, these may be non-adjacent tokens earlier or later in a sequence. \hl{move to early/mid}

% \section{Appendix ?: OV scores of Various Sequence Types}
% \label{appendix:OVscores}

% \textbf{OV scores of Various Sequence Types}

% \begin{figure*}[ht]
%   \centering
%   \includegraphics[scale=0.5]{plots/fig 5.pdf}
%   \caption{Month inputs on 7.11, Copy Score and top-5 tokens}
%   \label{copyScores_months} 
% \end{figure*}


% \section{Appendix ?: Test Prompts on GPT-2 Medium}

% \hl{postpone this}

\section{Circuit Entanglement and Editing Definitions}

\textbf{Definitions. } A \emph{circuit} can be defined as "a human-comprehensible subgraph, which is dedicated to performing certain task(s), of a neural network model" \citep{räuker2023transparent, wang2022interpretability}. To describe the specific graph representations of circuits we study in this paper, we define a \emph{circuit graph} as a connected graph $C$ with (1) a node set $N$ of components, and (2) an edge set $E$, in which an edge $(n_1, n_2)$ represents how component $n_1$ affects of component $n_2$. \footnote{This definition for circuit graphs is not a definition for circuits in general, but is one that is suited for the circuit graph representations and their figures that we discuss in this paper. } In this paper, we determine how a component affects another based on path patching, which we describe in \S \ref{sec:connMethods}. 
% \emph{circuit graph} (also referred to as circuit in this paper)
% \TODO{Not sure how this definition will be perceived. Perhaps either use the command definition or just remove this as state that "we define..."}

We define that a circuit graph $C$ is \emph{used} for a task $T$ based on how ablating all model components aside from those in the circuit still allows the model to have a certain level of performance; we determine this level as described in iterative pruning in \S \ref{sec:connMethods}. We note that a task $T$ can be broken into a set of sub-tasks $S_T = \{ S_1, ..., S_n \}$; for instance, one sub-task of IOI is to inhibit repeated subjects.

Next, we define a circuit graph $C_1$ to be a \emph{circuit subset} of circuit graph $C_2$ if all the nodes in the node set of $C_1$ are contained in the set of nodes for $C_2$. We also define $C_1$ to be a \emph{sub-circuit} of $C_2$ all the edges in the edge set of $C_1$ are also contained in the edge set of $C_2$. We further define circuit graph $C_1$ used for task $T_1$ to be a \emph{functional sub-circuit (or subset)} of circuit graph $C_2$ used for task $T_2$ if the following conditions are met:
(1) $C_1$ is a sub-circuit of $C_2$, and (2) $T_1$ is a subtask in $S_{T_2}$, the set of subtasks of $T_2$.

% 1) $C_1$ is a sub-circuit of $C_2$ 
    
% 2) $T_1$ is a subtask in $S_{T_2}$, the set of subtasks of $T_2$

% \begin{enumerate}
%     \item $C_1$ is a sub-circuit of $C_2$ 
%     \item $T_1$ is a subtask in $S_{T_2}$, the set of subtasks of $T_2$
% \end{enumerate}

% If condition (1) is met but not condition (

We further elaborate on the definition of circuit entanglement that will be used in future work involving model editing on shared circuits.

% \textbf{Feature Entanglement, Polysemanticity, and Superposition.} Polysemantic neurons, defined as neurons that activate highly on multiple unrelated features, has been observed in several studies \cite{nguyen2016multifaceted, 46832}. It is related to the phenomenon of superposition, which occurs when a model deals with representing more features than they have dimensions \citep{elhage2022superposition}. These concepts are also closely connected to the work of {\em feature vector entanglement} \citep{shen2020interpreting}, where editing one feature has an impact on another, and may be further linked to \emph{circuit entanglement}, a term that we define in \S \ref{sec:methods}.

\textbf{Circuit Entanglement.} Given that components play multiple roles \citep{merullo2023circuit}, it is clear that editing components in a circuit used for task A can have an effect on task B. Instead of just vaguely assuming this would have "some effect", such as ruining task B in "some way", our aim is to precisely describe, and thus approximately predict, what this effect is. We define two circuits $C_1$ and $C_2$ as being \emph{analogously entangled} if editing the functionality of $C_1$ affects the functionality of $C_2$ in an analogous way. For instance, let $C_1$ be for "digits continuation" and let $C_2$ be for "months continuation". If component $H$ in $C_1$ finds the "next digit of a sequence" and we edit it to now find the "previous digit", then if task B now finds the "previous month", we say $C_1$ and $C_2$ are \emph{analogously entangled}. 
\footnote[1]{We note that there are many cases where circuits are largely independent of one another in terms of editing, and also cases where editing one circuit will have an unclear effect on another. We aim to focus on cases where we can cleanly describe an entanglement effect. }


%%%%%%%%%%%%%%%%%
% In future work, we seek to expand upon shared circuits and entanglement effects for other tasks and models, and look for additional important components such as backup or inhibitory heads. Our aims include analyzing the effects of model editing on entangled circuits, quantifying the relationship between circuit entanglement and editing impact (which may be done via embedding space projection \citep{dar2022analyzing}), modifying the sub-circuit used for sub-task $S$ and observing if the ability to recognize $S$ in multiple tasks is destroyed, and editing a circuit used for task $S$ to perform a similar task $S'$, such as converting digits circuits to number words circuits or by utilizing a sub-circuit for one task to be re-used for another task (akin to the work of \cite{merullo2023circuit}). We also seek to test variations of existing methods, such as testing methods for ablating on combinations of components to find all possible circuits and paths for a task within a given threshold. Another topic we aim to investigate is in finding if there are any gradual changes from one circuit to another very similar circuit that works on a small task variation, such as in comparing differences between circuits of sequences with only digits versus circuits of sequences mixed with digits and other tokens.

% Analyzing the existence of similar or analogous circuits that exists across models is related to the topic of the universality hypothesis, which hypothesizes that similar representations exist across neural networks \citep{li2016convergent, kornblith2019similarity, olah2020zoom}. Studying larger models will also allow us to interpret circuits for more sophisticated sequence continuation tasks which GPT-2 Small did not succeed on, such as the Fibonnaci sequence, or comparing circuits for adding 2 (e.g. 2 4 6 8 10) vs circuits for multiplying 2 (e.g. 2 4 8 16 24).

% Additionally, open questions remain about the conditions that allow for or favor the existence of shared circuits entangled across similar inputs and tasks. This field of research also has the potential to contribute to transfer learning by possibly discovering methods of re-using components from previous, similar tasks when training on new tasks. This hypothesized type of transfer learning may reduce computing resource costs, which in turn reduces environmental harm. 
