# Supplementary material for: Towards Interpretable Sequence Continuation: Analyzing Shared Circuits in Large Language Models
Source: arXiv:2311.04131 source file (2024-10-04)
Supplement: Supplementary file 2 [file appendix_postponed.tex]

% \begin{table}
%     \centering
%     \begin{tabular}{c|c|c} 
%         \hline
%         \textbf{Model} & \textbf{No. Attn Heads} & \textbf{No. MLPs} \\
%         \hline 
%         GPT-2 Small & 144 & 12 \\
%         LLaMA 2 & 1024 & 32 \\
%         GPT-NeoX-20B & 2816 & 44 \\
%         \hline
%     \end{tabular}
%     \caption{Number of Components per Model \hl{(20B is too big; find smaller vers)} }
%     \label{tab:Number of Components per Model}
% \end{table}

\section{Appendix ?: Layer-wise Functionality Analysis}

% \subsubsection{Layer Output Analysis}

\textbf{Logit Lens.} Logits lens is a technique introduced by \cite{nostalgebraist2020interpreting} for understanding the internal representations of embeddings by unembedding each layer into vocabulary space and observing the top tokens. To assess the combination of neurons involved in a task, we perform logit lens on the sum of a combination of neurons. 

% \subsection{Logit Lens}
\subsection{Logit Lens Results}
We track how each layer changes the input. In Figure \ref{fig:logitlens}, we note that for the similar input tasks of digit sequence (1 2 3 4) and months sequence (January February March April), the correct token is found at layer 9. This supports the increasing sequence tasks sharing the head 9.1. We also note that early layers do not seem to output tokens that are relevant to the correct token type, such as digit or month. Logit lens can be taken for every token in the sequence; here, we only show the logit lens for the last token.

\begin{figure}[ht]
  \centering
  \includegraphics[scale=0.35]{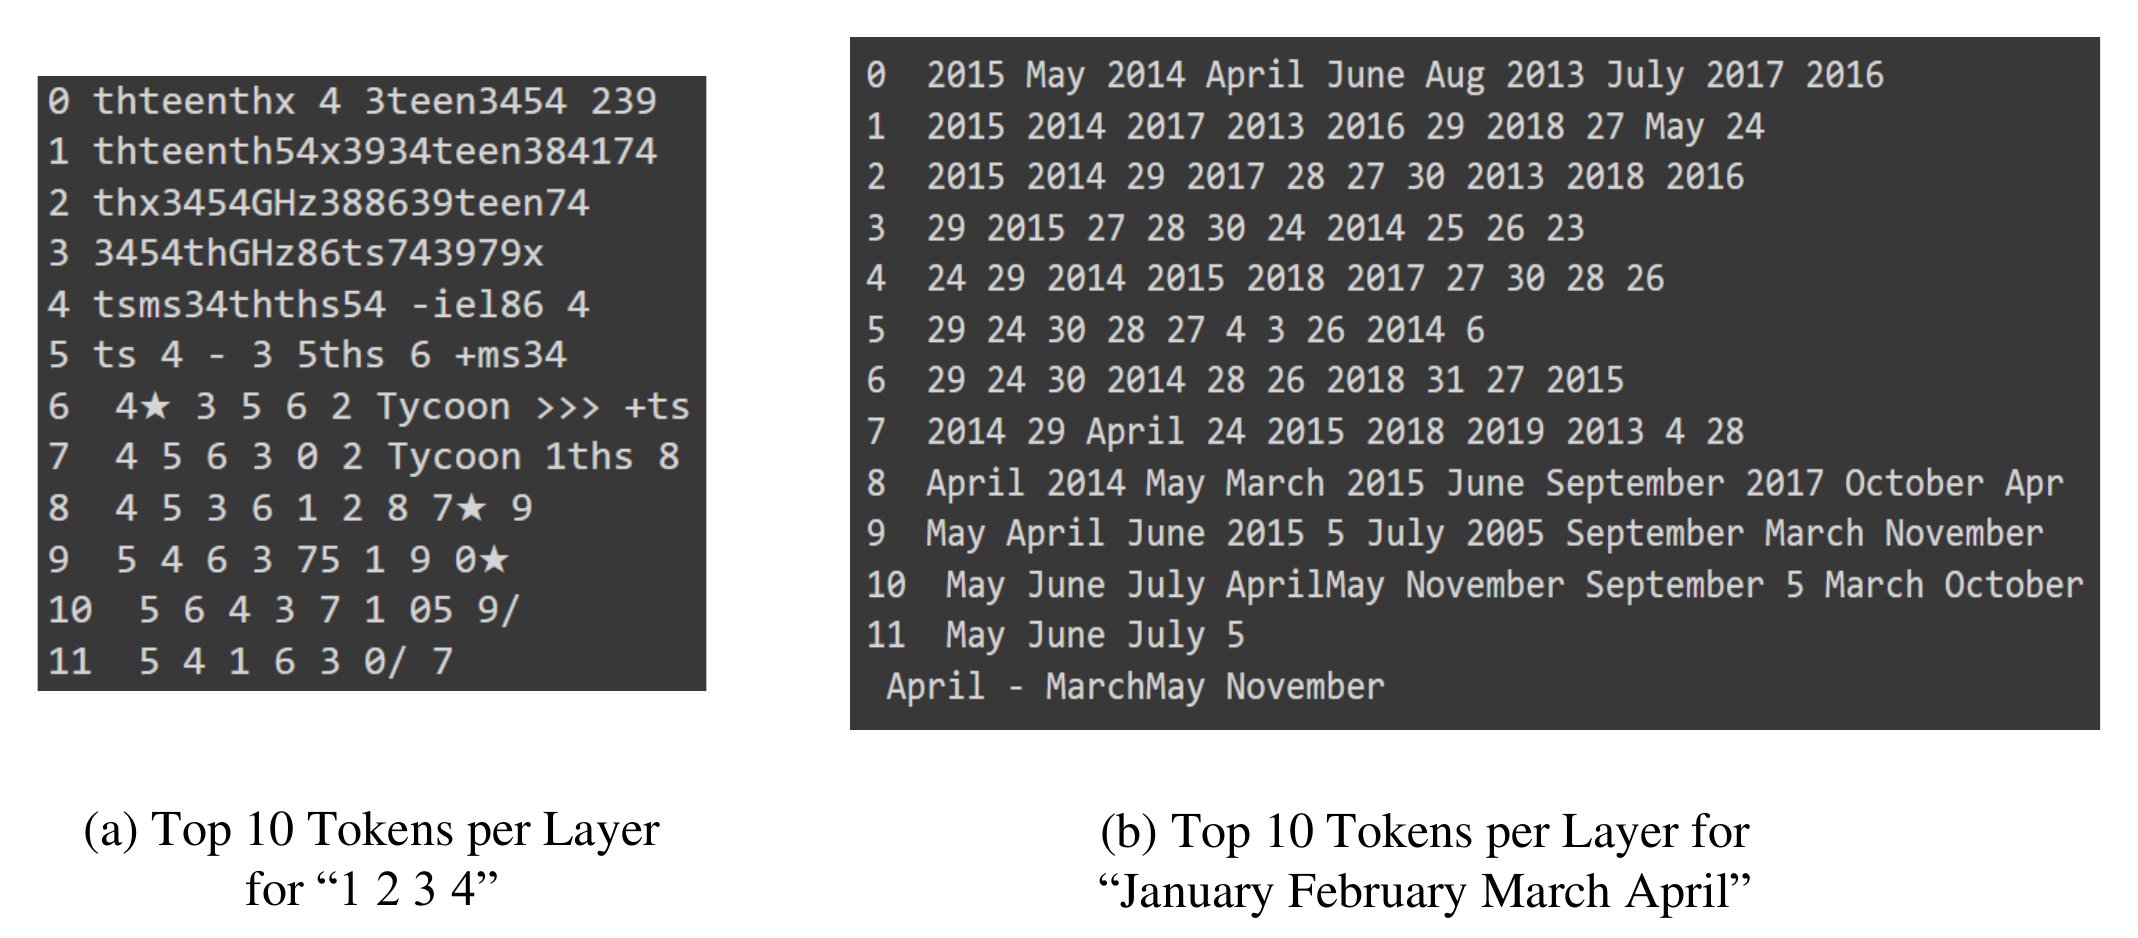}
  \caption{(a) Unembedding of the top 10 tokens for each layer of the sequence "1 2 3 4" (b) Unembedding of the top 10 tokens for each layer of the sequence "January February March April"
  }
  \label{fig:logitlens}
\end{figure}


\section{Appendix ?: MLP Analysis}
\label{appendix:MLP}

\textbf{SVD for Interpretable Directions.} The Singular Value Decomposition, or SVD, of a weight matrix has been used to find singular vectors, or directions, that correspond to interpretable features in LLMs \citep{millidge2022singular}. Thus, we adapt the techniques they developed to our work. In particular, we utilize the approach of auto-labeling these directions using GPT-4 with instruction prompts we design to allow the model to identify concepts related to agents.

To find interpretable directions, each component of the right singular matrix is unembedded into vocabulary space, which gives the tokens with the highest values. Taken together, these top tokens often correspond to a semantic concept, such as “animals”. Our analysis was performed on the MLP input weight matrices. This process traces how MLP neurons react to semantic features like numbers to identify key components of sequence circuits. 

\emph{GPT-4 Auto-Labeling. } \cite{millidge2022singular} proposed auto-labeling each singular vector by inputting their top-15 tokens, along with an instruction prompt, into GPT-3. In this paper, we perform this method with GPT-4. Instead of using an instruction prompt to label directions with interpretable concepts, we check if a direction contains concepts corresponding to a desired sequence type. 

\hl{[instead of autolabeling, we can also use neuron-to-graph and/or neuroscope]}

\subsection{MLP Patching and Neuroscope Results}

% [This section may be rmv / move to appendix as it doesn't directly interact with hypothesized circuit]

We utilize activation patching on individual neurons to find important neurons, as displayed in Figure \ref{mlp_actvpath}. Using multi-prompts for digits, we look at L9 and L10 to find two that stand out as “number neurons” (their contribution is partial, so combinations of neurons are likely involved):
\begin{itemize}
\item Layer 9: 934 
\item Layer 10: 1721 
\end{itemize}

\begin{figure}[H]
% \begin{figure}[ht]
  \centering
  \includegraphics[scale=0.5]{plots/fig 7.pdf}
  \caption{Activation Patching by Neuron for L10. Neuron 1721 stand out as having more than 0.2 patch improvement
}
\label{mlp_actvpath}
\end{figure}

Neuroscope supports these findings by showing its strong activations near number-type tokens, as seen in Figure \ref{fig:neuroscope}.

\begin{figure}[H]
% \begin{figure}[ht]
  \centering
  \includegraphics[scale=0.4]{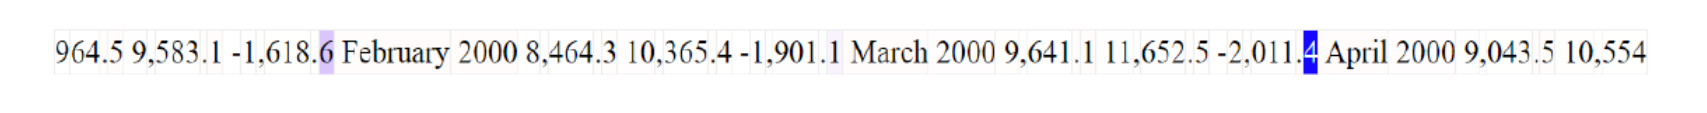}
  \caption{A max activating example from the dataset for L10, N1721
}
\label{fig:neuroscope}
\end{figure}

\subsection{SVD Analysis}

To lessen the amount of API calls, we note that \cite{millidge2022singular} stored whether a singular vector was interpretable by the model or not. Thus, we only consider vectors that were already labeled in the previous study as interpretable.

MLP weight matrix singular vectors are stated to be more polysemantic and less interpretable than attention head OV weight matrix singular vectors. As such, a concept must share a direction with other concepts. We analyze MLP input weight matrices.

We note that X out of X, or around X\%, singular directions are labeled as interpretable, and X out of X, or around X\%, of these interpretable directions are found to correspond to [seq type] concepts.
