# Supplementary material for: Towards Interpretable Sequence Continuation: Analyzing Shared Circuits in Large Language Models
Source: arXiv:2311.04131 source file (2024-10-04)
Supplement: Supplementary file 3 [file appendix_temp.tex]

\section{Results on Larger Models}

\TODO{Instead of using autoencoders/steering, compare between multiple models}

Plan Draft:
\begin{itemize}
    \item train toy models (1L, 1 attn head, etc) on seq cont. 
    \item auto ablate circs on 246, 248, on gpt-neoJ-6B
    \item transfer activations from one model to another
    \item modify algo to patch by pos, too
    \item use KL div
\end{itemize}

toy model training: The training data and testing data will have no overlaps. However, it is expected that the model must encounter I+1 one after I in training samples, as it inherently doesn't know how the number tokens are ordered.

--------

%%%%%%%%%%%%%%%%%%%%%%%%%%%%%%%%%%%%%%%%%%%%%%%%%%%%%%%%%%%%
reviewer notes:
immediate comments on the paper:
1- make table col names bold
2- use the same font for text ad figs
3- add some concreate future directions 
4- add broader impact statement - how can this work be used and how can it be misused?
remove footnote 5.


One of the main concerns is that the model is only valid for sequence continuation on small samples of data (eg. there are only 12 months to use, and it doesn’t go past twenty for number words), so there is not enough data

A second concern is that sequence continuation is more "memorization" of what number comes next, rather than generalization. I'm not sure if there's a way we can get around that, unless we do something like train a toy model on sequence continuation and try to apply it to a new case (eg. train on 1 2 3 4 and some 2 4 6, then apply it to never before seen seqs like 10 12 14; or train on some numbers seqs but only number word "one next" (len 2 seqs), then apply to never before seen number word seqs, etc.) That seems sort of arbitrary though

%%%%%%%%%%%%%%%%%%%%%%%%%%%%%%%%%%%%%%%%%%%%%%%%%%%%%%%%%%%%
% \section{Decomposing Steering Vectors}

% \TODO{Currently looking into seeing if steering vectors and sparse autoencoders can be used for this topic}

% Plan Draft:
% \begin{itemize}
%     \item Generate steering vector by averaging the differences in intermediate residual stream activations after a transformer block given paired X / non-X texts (where X is a type, such as digits vs number words)
%     \item test this steering vector on random token types types
%     \item test the relevant token dataset on random vectors
%     \item add with coefficient (scaling) and subtract
%     \item use these as 'model editing' to turn numbers into number words, etc. (may need larger model)
%     \item Run prompts thru llama2 (huggingface after meta permissions, TPU) using larger dataset of +2, +3, etc. interval sequences. Compare to Pythia models.
%     \item embed both llama2 and pythia model activations in embedding space and measure distances
% \end{itemize}

% \subsection{Decomposing Shared Activations}

% We run our similar tasks through the model and collect their activations. 

% \subsection{Feature Ablation Experiments}

% After decomposing

% We ablate MLP features and observe how they affect downstream tasks. This is performed by processing the input up through the MLP layer, then passing its activations to the autoencoder, which calculates feature activations. Afterwards, for each token in the context, the product of the feature direction and its activation is subtracted from the MLP activation to perform zero ablation. Finally, the forward pass is completed.
