# Supplementary material for: Towards Interpretable Sequence Continuation: Analyzing Shared Circuits in Large Language Models
Source: arXiv:2311.04131 source file (2024-10-04)
Supplement: Supplementary file 4 [file old_appendix.tex]

\section{Appendix: (Unfinished Draft to be Completed Later)}

\subsection{Definitions}

In order to define when members of a set of sequences are all analogous with one another, we present a definition of analogy that is based on the \textcolor{blue}{\textit{"match"}} definition used for the structure-mapping engine \citep{FALKENHAINER19891}. 
First, to define how concepts relate to one another, we provide the definition of a \textcolor{red}{\emph{semantic network}} \citep{sowa1992semantic}. 

\begin{definition}[\textcolor{red}{Semantic Network}]
A semantic network is a tuple \( S = (V, E, P, Q, L_v, L_e) \), such that:

\begin{align*}
    &\textcolor{green}{V} \text{ is a non-empty set of vertices, each representing a concept} \\
    &\textcolor{green}{E} \subseteq \textcolor{green}{V} \times \textcolor{green}{V} \text{ is a set of ordered pairs of vertices, representing the relations between concepts} \\
    &\textcolor{purple}{P} \text{ and } \textcolor{purple}{Q} \text{ are sets of features} \\
    &\textcolor{orange}{L_v}: \textcolor{green}{V} \rightarrow \textcolor{purple}{P} \text{ is a labeling function that maps each vertex in } \textcolor{green}{V} \text{ to a concept feature } \textcolor{purple}{p} \in \textcolor{purple}{P} \\
    &\textcolor{orange}{L_e}: \textcolor{green}{E} \rightarrow \textcolor{purple}{Q} \text{ is a labeling function that maps each edge in } \textcolor{green}{E} \text{ to a relation feature } \textcolor{purple}{q} \in \textcolor{purple}{Q}
\end{align*}
\end{definition}


For the ease of working with experiments, we investigate sequences such that each concept is mapped to a single token; in general, each concept may be represented by multiple tokens, where each token may not correspond to a concept at all. Thus, the set of concepts $V$ of a semantic network can be implicitly represented by a token sequence $t$ that contains $V$. 

\textbf {[ The following is an idea under development and is not rigorously defined yet; it may take time to rigorously review and thus may be postponed for a later paper. This is put here just as a starting point to brainstorm more ways to measure vectors during experiments by translating these defs to code. The paper to submit soon will focus on experiments rather than this definition. ]}

Note that the feature labeling functions are not present in the token sequence $t$; another function that processes $t$ would have to "assign" these features by mapping each token into the latent space of a layer. Transformer models represent each token as an embedded vector
\citep{NIPS2017_3f5ee243}.(refine citation to- GPT specific), and features  are often loosely defined as vectors, which are a linear combination of neurons, each being a dimension in latent space of a layer \citep{gurnee2023finding}.

Therefore, one such "labeling" would be to define concept features as vectors in latent space, and to measure "labeling" as the distance, calculated via cosine similarity, from a token embedding vector to a feature vector. Each layer would transform the initial token embedding vector into a new vector in a new vector space. The cosine similarity would not just map a concept vector to a feature vector, but calculate, via dot product, the normalized projection value of how strongly that concept is measured by a feature. 

From this definition, we would not need to separately represent edges or require an edge labeling function, as a relation between two concept vectors can be measured as their vector difference projected onto a "relation feature vector dimension". [actually it might still be helpful to explicitly state which relation feature dims we want to measure, so this should probably still be stated]

To better describe a semantic network as represented by a neural network, we introduce the following definition:

\begin{definition}[\textcolor{blue}{Relational Representation}]
A relational representation is a tuple $ R = (V, P, L)$, such that:
\end{definition}
\begin{align*}
    &\textcolor{green}{V} \text{ is a non-empty set of vectors, each representing a concept} \\
    &\textcolor{purple}{P} \text{ is a set of feature vectors } \textcolor{purple}{P} \subseteq \textcolor{green}{V}, \text{ which form a subset of the latent space } \textcolor{green}{V} \text{ of a layer} \\
    &\textcolor{orange}{L}: \textcolor{green}{V} \times \textcolor{purple}{P} \rightarrow  \mathbb{R} \text{ is a function that outputs the cosine similarity of each vector in } \textcolor{green}{V}\\
    & \text{ with every feature vector } \textcolor{purple}{p} \in \textcolor{purple}{P}
\end{align*}



In contrast to a semantic network, the labeling function does not just map one object to another object, but it maps an object to a value between 0 and 1 in a dimension. 

The subset $P$ may be thought as as a filter, or a slice. In other words, we are only selecting certain feature dimensions to compare similarity on (and the set of all feature vectors $P$ may not form a basis and does not necessarily span a latent space of a layer.) Additionally, we may just consider $V$ and $P$ as "one set of vectors", as concepts may be considered as features, and vice versa. However, we separate the two here for explanation purposes, as we can refer to $P$ as the "level of abstraction" from which we want to measure analogies from. For instance, a red plant and a pink moose are not similar in the "species" dimension levels, but they are similar if we select the "color" dimension levels to perceive them from.

NOTE: Features are still fuzzily defined, so this attempts to give it more definition.
(to put in bib file):
https://www.lesswrong.com/posts/LNA8mubrByG7SFacm/against-almost-every-theory-of-impact-of-interpretability-1

Next, we aim to define an analogy between two relational representations.

\begin{definition}
\label{def:an_reln}[Analogous Relational Representations] {\em A relational representation $R_1 = (V_1, P_1, L_{1})$ is considered} analogous {\em to another relational representation $R_2 = (V_2, P_2, L_{2})$ if there exists a (not bijec?) function $f_1: V_1 \to V_2$ and a function $f_2: P_1 \to P_2$ such that for (every?) vector $v_1 \in V_1$ and $p_1 \in P$, and for a selected threshold $\epsilon$: 

\[ \left| L_1(v_1, p_1) - L_2(f_1(v_1), f_2(p_2)) \right|  \leq \epsilon \]
}

\end{definition}

The user-selected threshold $\epsilon$ measures the "abstraction strength" in the analogy. This may be adjusted differently for each $v$ to $p$ mapping. A loose analogy- for example, - would have a large $\epsilon$, while a strict analogy would require a smaller $\epsilon$ for two representations to be considered analogous.

\textbf{Example.} Consider a set of vectors representing concepts of a brain, $\{$  long term memory, working memory, hippocampus $\}$, and another set of a vector representing concepts of a computer, $\{$  hard drive, RAM, disk controller $\}$. 

(this is a BIG assumption that reqs evidence)
Additionally, we may assume there's a circuit which processes how the brain concepts interact to project onto "relational feature" vectors for writing long term to short term memory, and likewise, there's a circuit that does the same for writing data from RAM to the hard drive.

If we construct a map $f$ such that f(long term memory) = hard drive and f(short term memory) = RAM, we should ensure that their interactions which project onto the "relational feature" vectors will be similar to the concepts after this function $f$.

[put the above exm in a diagram]

---

[ NOTES: This is where the definitions must be refined as they poorly capture what it means to "go through a circuit to project onto vectors measuring relational interactions between features".

Overall, this definition of an analogy measures how much relational similarity two vector space representations share under a mapping (a lot of existing literature probably already has better ways to do this, though not sure if suited for this task. see- determinant, etc).

Path-based similarity may also be useful to try to define. That is, we are not just interested in aggregating then comparing "one off" edge matches, which ignores the graph topology of how edges connect with each other. To account for the graph topology similarity, one can compare paths between analogous representations.

This is measuring analogous representation of input sequences. However, we may need to separately define an analogous representation for CIRCUITS within a model (in a later paper, extend to between models- see model-to-model section). ]

---

There is another perspective to think about this from. If we define $L(v)$ as the cosine similarity between vector $v$ and every feature vector $p$ (perhaps by taking their average, which is bad if you're measuring them separately), we can think about the analogy criteria as requiring, for every element $v \in V$:
\[
f(L_1(v)) \approx L_2(f(v)).
\] 

NOTE: This is not a good way to state this. Additionally we cannot take f(L(v)) because f maps vectors, whereas L(v) is a scalar. An alternative way is to have $L$ map v not to the cosine similarity value, but to the vector projection of v along p, $proj_p(v)$. That way, $L_p(v) \in P$. Then, we can measure how close $f(proj_{p_1}({v_1}))$ is to $proj_{p_2}({v_2})$, as both are in vector space $P_2$. It is still under consideration whether to use L(v,p), or L(v) for every p, or $L_p(v)$, etc. when mapping to $P$.

This can be expressed by a commutative diagram:

\[
\begin{array}{ccc}
\textcolor{green}{V_1} & \xrightarrow{\textcolor{orange}{L_1}} & \textcolor{purple}{P_1} \\
\downarrow f & & \downarrow f \\
\textcolor{green}{V_2} & \xrightarrow{\textcolor{orange}{L_2}} & \textcolor{purple}{P_2}
\end{array}
\]

% V_2 & \xrightarrow{L_2} & \mathbb{R}

---

Next, we define continuing sequences in natural language in terms of relational representations, showing that this leads to analogous continuing sequences. Since the common "level of abstraction" are the natural numbers, we will define $P$ using natural numbers, with each $n \in \mathbb{N}$ encoded as an embedded vector. Then, a continuing sequence is considered as analogous to the natural numbers if it satisfies Definition \ref{def:an_reln}.

Let \( ( \mathbb{N}, +) \) denote the set of natural numbers with the usual addition operation. We can define the successor function \( S: \mathbb{N} \to \mathbb{N} \) by
\[
S(n) = n + 1.
\]
\( S \) is an endomorphism of \( \mathbb{N} \), since it maps \( \mathbb{N} \) to itself while preserving the addition operation.

% on \( \mathcal{T} \) such that
% \[
% T(t_1) = t_2, \quad T(t_2) = t_3, \ldots, \quad T(t_n) = t_1.
% \]

[this section needs to show sequences in terms of the prev defs]

We map each single token concept to an embedded vector. A sequence $f$ is inherently a function from the natural numbers to a set X that defines an ordering on the set X.

We want to define a function \( f: \mathcal{T} \to \mathbb{N} \) that captures the ``successor" relationship between these tokens, similar to the \( +1 \) operation on \( \mathbb{N} \).

Define \( f \) as follows:
\[
f(t_1) = 1, \quad f(t_2) = 2, \quad \ldots, \quad f(t_n) = n.
\]
We define a successor operation \( T: \mathcal{T} \to \mathcal{T} \) on \( \mathcal{T} \) such that
\[
T(t_1) = t_2, \quad T(t_2) = t_3, \ldots, \quad T(t_n) = t_1.
\]

The function L measures how similar each member of a sequence is to its corresponding natural number.

[ ISSUE: Is this even represented in a neural network? We need evidence that shows Jan and 1 somehow map to each other along certain feature directions. This is not seen in individual neurons yet; so it may be in a linear combination of neurons (see superposition), possibly of polysemantic neurons. Thus, if no evidence of this is found, these definitions must be drastically reworked. This is where our search algorithms will be used to find combinations of neurons that may represent this "common, abstract feature" that measures how similar Jan and 1 are. The same or a different feature may measure Feb and 2, etc. ]

[ to be continued later ]

---

Lastly, we extend this definition to a set of multiple token sequences.

\begin{definition}[Set of Analogous Sequences] {\em Members of a set of token sequences are} analogous {\em with one another if every member is analogous with a (shared P? or shared sequence?)} [...use $\sim$ from eqv class here]

\end{definition}

Once this definition is better defined, depending on the space, it may be proven that by transitivity, every member in the set is analogous with one another through the "shared abstraction" that "canonically represents the set". 
Then, a set of analogous relational representations would all be similar in certain dimensions.

The reason for defining a set of analogous sequences is to define a class of "children" to a more abstract parent concept. Set membership is defined by conditions. Then for experiments, we can show that all members of an "abstract class" also correlate with some property of a sequence. Experimentally providing evidence of correlations with abstract classes and circuits will demonstrate why this definition is useful, as it represents an actual pattern that can be studied.

\subsection{Identifying Shared Neurons with Analogous Features}

Idea: Use neuron2graph to identify important neurons by searching for them using feature search terms?

ISSUE: It seems like MLP neurons are not important for this circuit. We may look at shared circuits for other inputs instead of narrowing down to just sequence completion.

\subsection{Neuron Combination Selection Algorithm}

[sparse probing can already show layers using combinations of neurons so this is probably not needed if it does worse]

[this is a placeholder algorithm for a crude, ineffective starting point; a better algorithm will replace it as this paper is developed]

Greedy algo for ablating neuron combos and neuron+heads combos:

try both bottom-up and top-down.

1. Use neuron2graph/etc tool to find important neurons. Or get scores by ablating them and measuring logit difference between correct and incorrect token.
\\
2. Find neuron with biggest logit restoration score, and ablate it with the neuron with next highest score. 
\\
3. Continue adding them until the restoration score contribution is "not significant enough" relative to a fraction of the total score.

\begin{algorithm}[!thbp]
 \rule{\linewidth}{.5pt}

 \begin{flushleft}
\emph{Input:} $\mathcal{N}$, a list of neurons, model $M$, input tokens $I$, originalScore, scoreThreshold

\emph{Output:} $\mathcal{O}$, a subset of neurons
\end{flushleft}

\begin{small}

\algsetup{linenodelimiter=.}
  \begin{algorithmic}[1]

\STATE Initialize $\mathcal{O}$ as an empty list; 

\FOR{every neuron $n \in \mathcal{N}$}

\STATE Run inputs $I$ through model $M$ with mean ablation hook on $n$

\STATE ablatedScore = correctLogitScore - incorrectLogitScore 

\IF{originalScore - ablatedScore < scoreThreshold}

\STATE Add neuron to $\mathcal{O}$;

\ENDIF

\ENDFOR

\STATE add rest of algorithm later

\end{algorithmic}

\end{small}

\caption{Algorithm {\em
FindNeuronSubset}}
\label{alg}

\end{algorithm}

\subsection{MLP and Attention Head Circuit Discovery}

NOTE: this has been done before. 

TO CITE: https://arena-ch1-transformers.streamlit.app/[1.4]\_Balanced\_Bracket\_Classifier

We assess a method to determine the interactions between MLPs and Attention Heads. MLPs are said to associate input to output information, and attention heads are said to move information. Thus, we hypothesize that there exist circuit algorithms which move information to MLPs, which then process them to new outputs.

A previous study \citep{wang2022interpretability} uncovered an algorithm called "Indirect Object Identification" in which, given a sentence containing an indirect object and other subject, the GPT-2-small model would correctly identify the duplicate subjects, and choose the non-duplicate subject, the indirect object, as the next token to predict with the highest logit. This was done by a circuit of attention heads that identified the subjects, moved them by copying to the output of certain heads, and inhibited the incorrect subjects in order to have the correct subject have the highest logit. In this algorithm, no new information needs to be outputted as the correct answer, as it simply copies existing information from the input token sequence.

In other cases, new information must be produced as the correct answer. For instance, in the case of continuing sequences, the model must find a way to choose the next member of the sequence by looking at the last few members of a sequence. Thus, we hypothesize that there are key-value stores in which the model takes in the last element and outputs the next successive element. Moreover, we hypothesize that the circuit which does this for natural numbers may be similar to the circuit which does this for other continuing sequences.

\subsection{Model-To-Model Comparison}

In previous sections, we compared components that activated for analogous input sequences. In this section, we use the same input sequences on different models to see if there are analogous circuit components between models.

\subsubsection{Comparison to GPT-2 Medium}

We compare running the input sequence “2 4 6 8 10 12” on both  GPT-2 Small and GPT-2 Medium. Attention heads that attend to tokens further back than previous token are of interest to observe if sequences are recognized based on members of the sequence that are further back than the previous token.

We notice that in GPT-2 Medium, head 11.4 attends from the last token "12" to token “6”, which is three tokens back. This is similar to head 6.1 in GPT-2 Small attends from the last token "four" to token "two", which is two tokens back.

\begin{figure}[H]
% \begin{figure}[ht]
  \centering
  \includegraphics[scale=0.5]{plots/6.1 small vs 11.4 med.pdf}
  \caption{(a) Head 6.1 for GPT-2 Small vs (b) Head 11.4 for GPT-2 Medium
}
\end{figure}

Attention Head Patching discovers that GPT-2 Medium has a head 19.1 that is very important. It may be the case that 9.1 from Small and 19.1 from Medium perform similar functions, as both are very important late heads. [show figure].

[ Future plans to do: Show that these sub-circuit components are analogous across models by showing knocking these sub-circuits will result in analogous performance changes. Not only that, but combos of sub-circuits knocked out will have analogous effects, both when out and when restored. This may be saved for a follow-up paper]
